# Supplementary material for: Gaia Data Release 3: Ellipsoidal Variables with Possible Black-Hole or Neutron Star secondaries
Source: arXiv:2206.06032 ancillary file (2022-06-13)
Supplement: Supplementary file 1 [file GaiaEllip_supplementary.pdf]

*Astronomy & Astrophysics* manuscript no. output ©ESO 2022
June 12, 2022

# *Gaia* Data Release 3

## Ellipsoidal Variables with Possible Black-Hole or Neutron Star secondaries - supplementary material

R. Gomel[1], T. Mazeh[1], S. Faigler[1], D. Bashi[1], L. Eyer[2], L. Rimoldini[3], M. Audard[2], N. Mowlavi[2,3], B. Holl[3], G. Jevardat[3], K. Nienartowicz[3], I. Lecoeur[3], and L. Wyrzykowski[4]

[1] School of Physics and Astronomy, Tel Aviv University, Tel Aviv, 6997801, Israel
e-mail: roygomel@tauex.tau.ac.il

[2] Department of Astronomy, University of Geneva, Chemin Pegasi 51, CH-1290 Versoix, Switzerland

[3] Department of Astronomy, University of Geneva, Chemin d'Ecogia 16, CH-1290 Versoix, Switzerland

[4] Warsaw University Astronomical Observatory Department of Physics Al. Ujazdowskie 4 00-478 Warszawa Poland

June 22

### 1. *Gaia* *G*-band light curves of our candidates

This section presents folded *Gaia* light curves in the *G* band of the 262 candidates with $\hat{q}_{\rm min}^{-1\sigma} > 1$, in descending $\hat{q}_{\rm min}$ order. For each candidate, the *Gaia* DR3 identifier (id), together with the *Gaia* period in days and the value of $\hat{q}_{\rm min}$, are given, and a three-harmonics model is plotted with a solid red line.

### 2. Data table of our candidates

Given below a summary table containing results of the analysis performed on our 262 candidates with $\hat{q}_{\rm min}^{-1\sigma} > 1$, in descending $\hat{q}_{\rm min}$ order. The table includes the *Gaia* DR3 id, *Gaia* orbital period, reference time $T_0$ [BJD-2455197.5] which was chosen so that $a_{2s} = 0$, average G magnitude $\overline{G}$, and cosine and sine Fourier coefficients $a_{ic}, a_{is}$ $\{i = 1, 2, 3\}$ of the three-harmonic model, defined by equation (1), each with its uncertainty. The table also gives the total number of *G*-band FoV transits, the derived mMMR and the lower-percentile mMMR. Additional details are found in the paper, and the table is online available at the CDS.

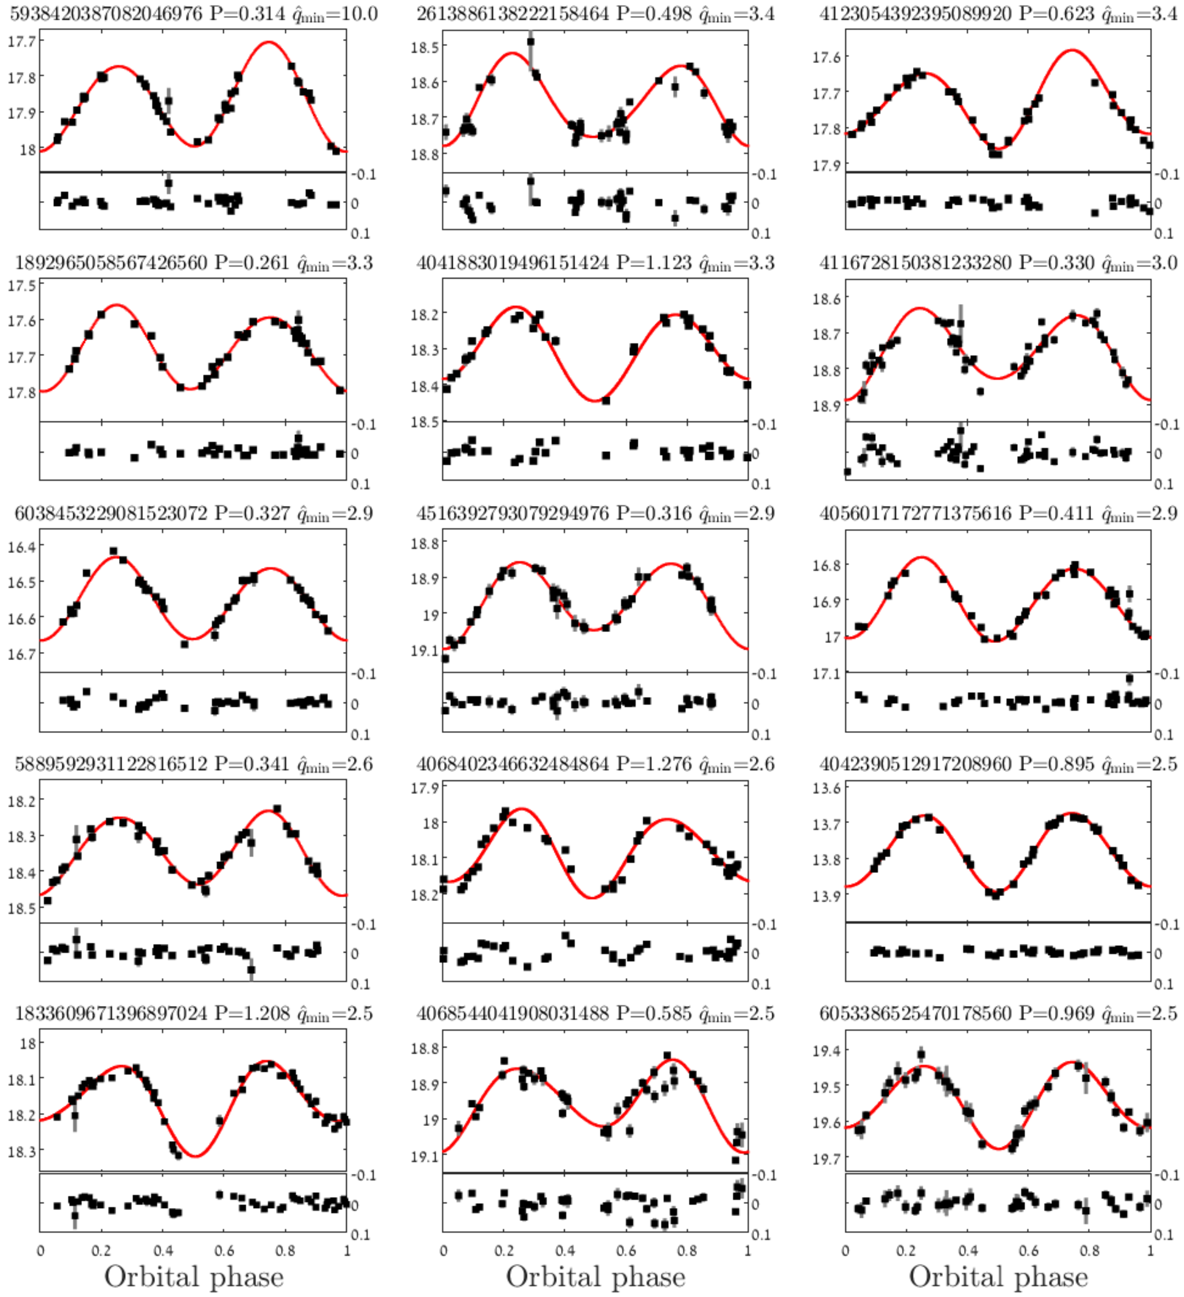


Fig. S1: Folded *Gaia* light curves in the *G* band of the 262 candidates in descending $\hat{q}_{\rm min}$ order. For each candidate, the *Gaia* DR3 id, together with the *Gaia* period in days and the value of $\hat{q}_{\rm min}$, are given. The epoch of the second-harmonic minimum corresponds to phases 0 and 0.5, and a three-harmonics model is plotted with a solid red line. All curves are plotted with a mag range of 0.4, for convenience. The residuals are plotted in the lower panels and are shown between -0.1 to 0.1 mag for clarity.

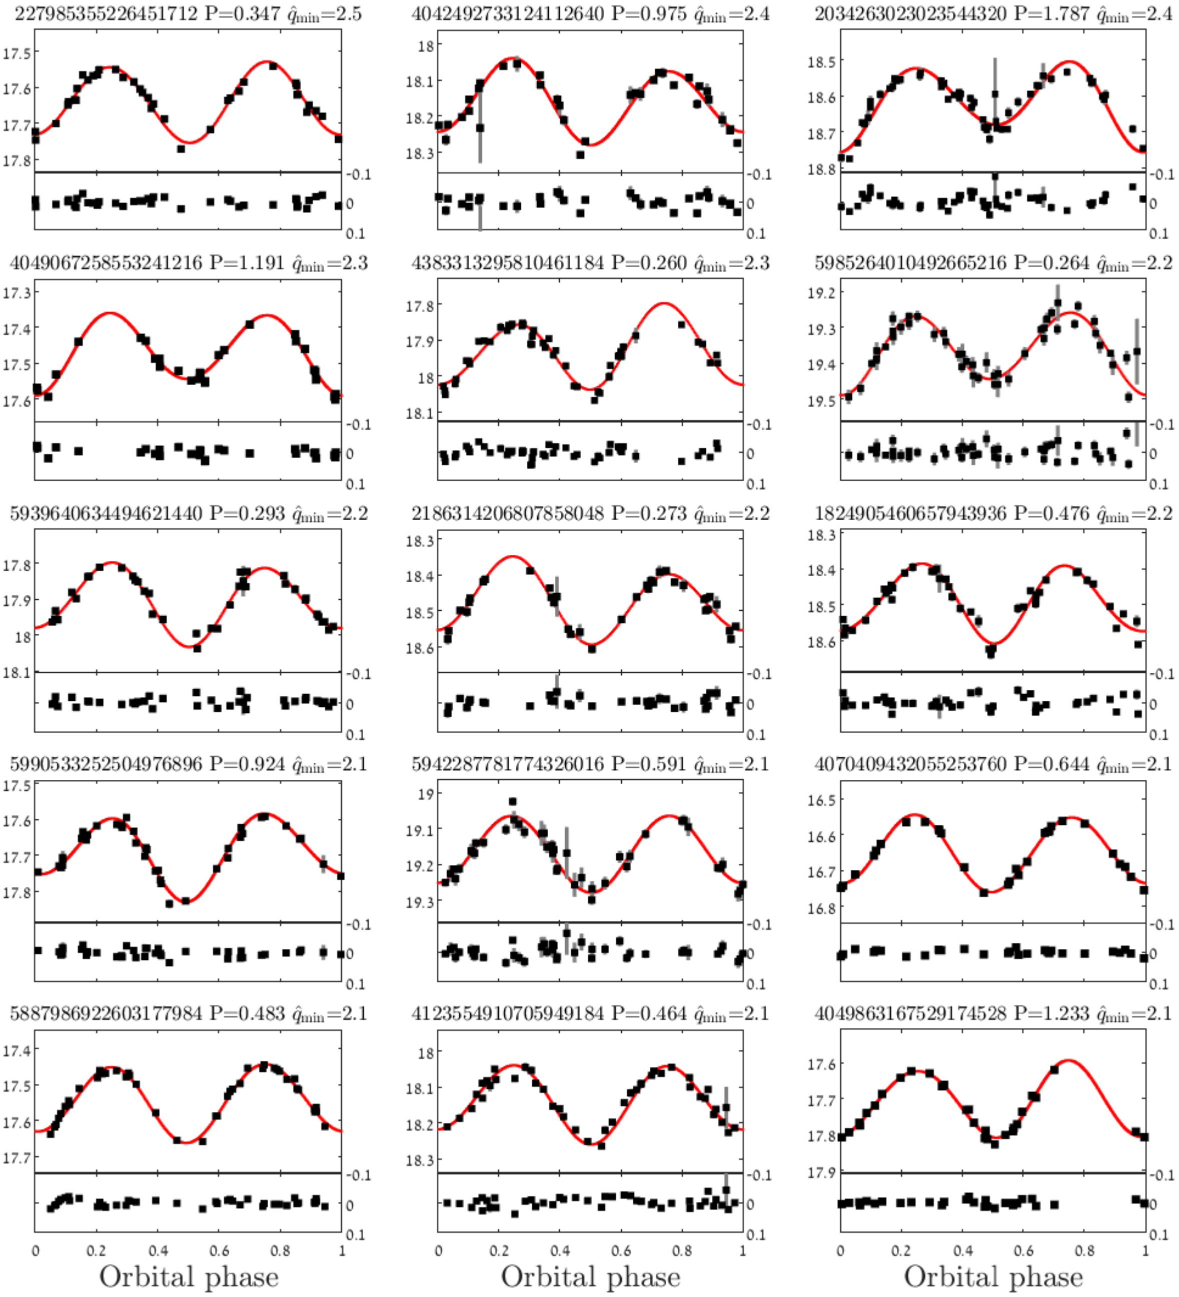


Fig. S1: Continued

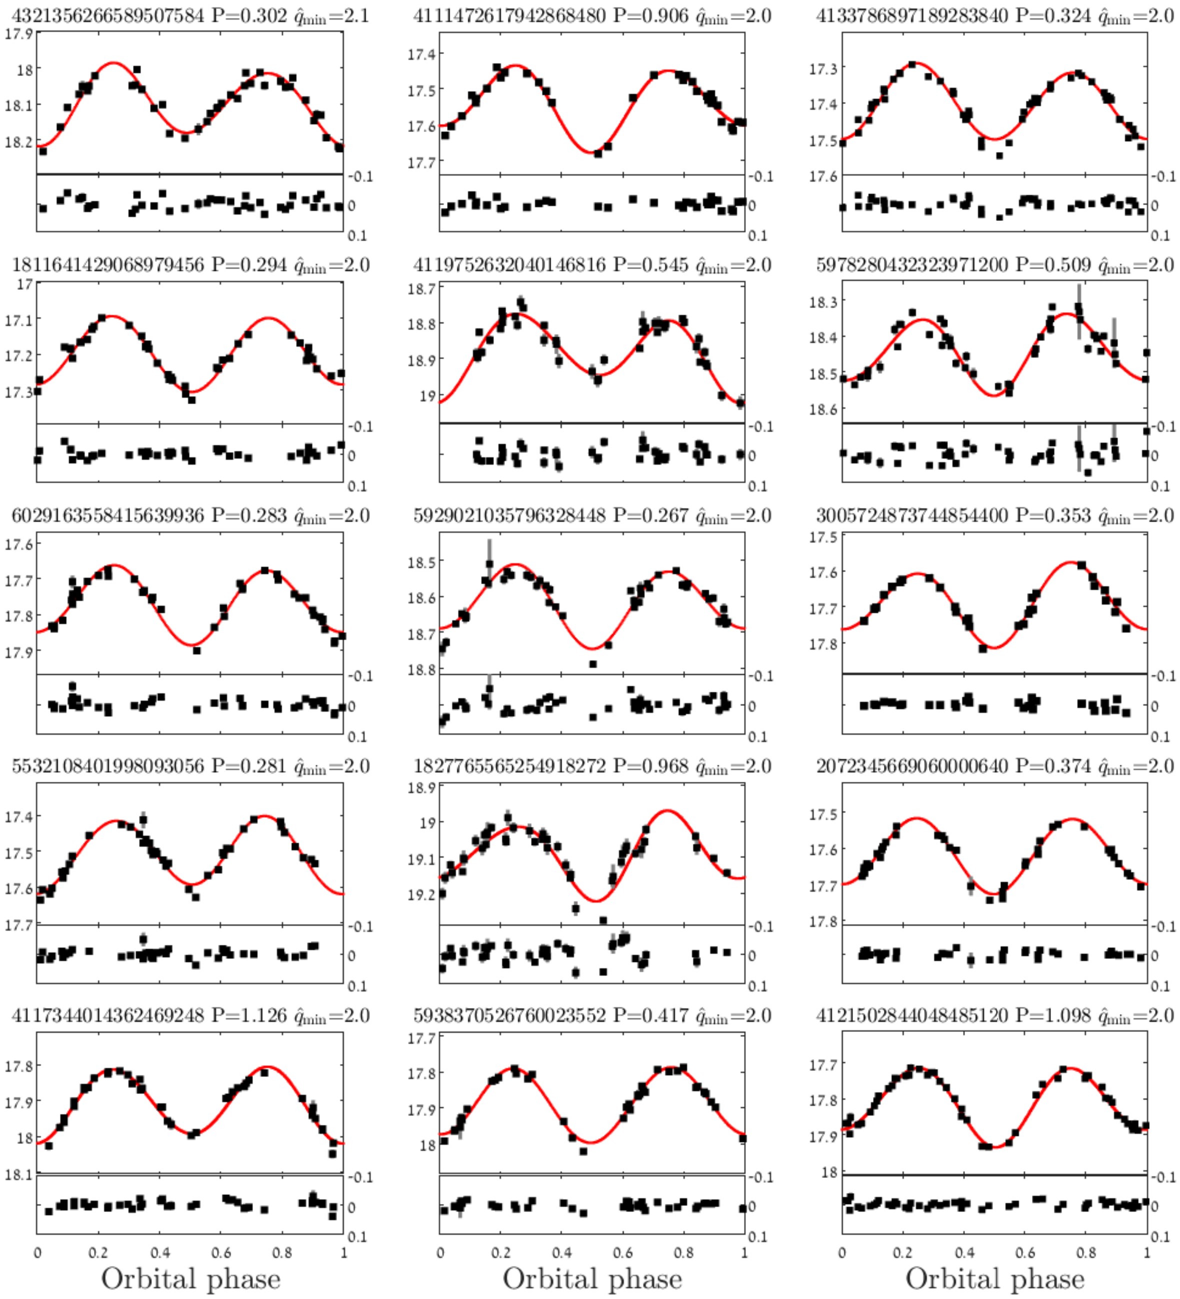


Fig. S1: Continued

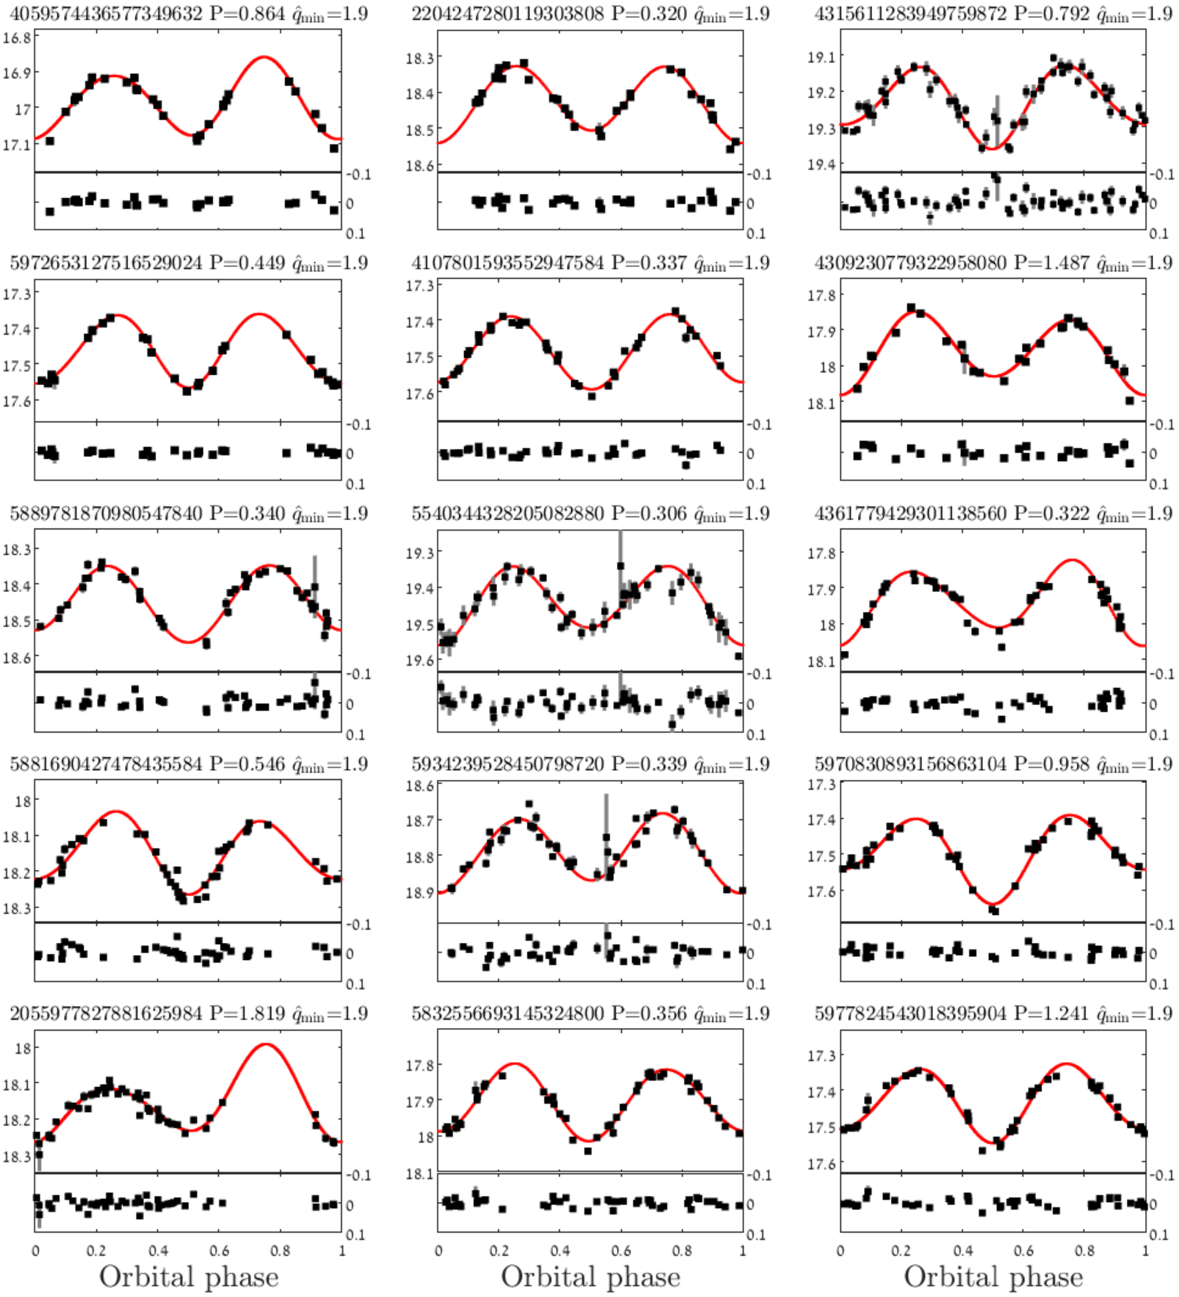


Fig. S1: Continued

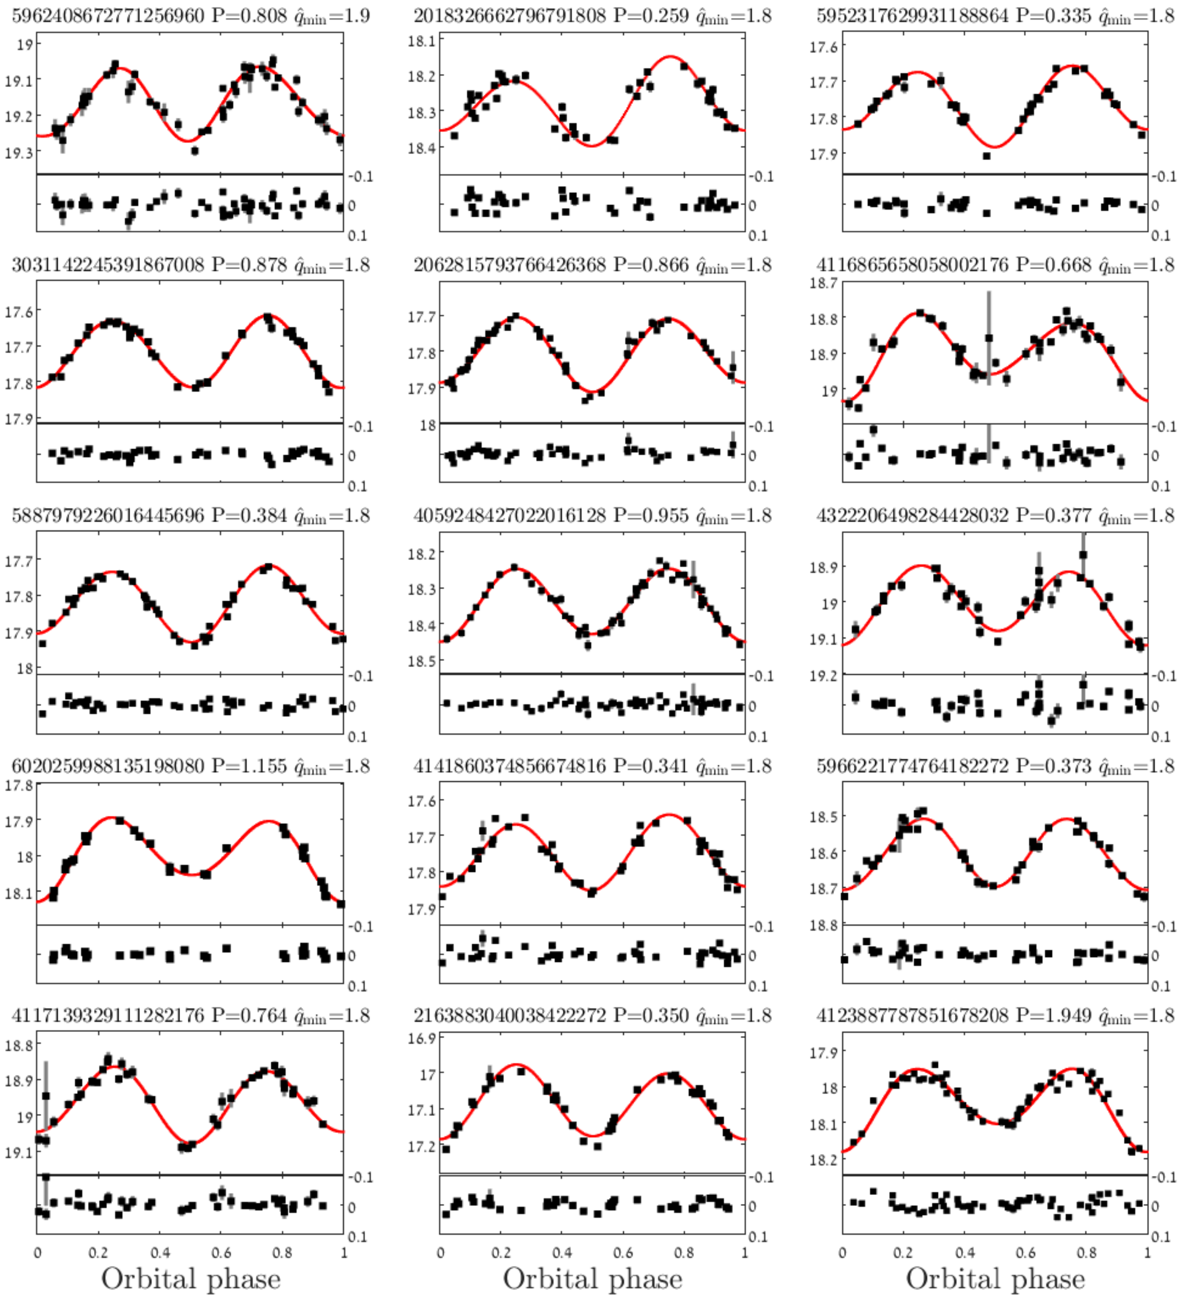


Fig. S1: Continued

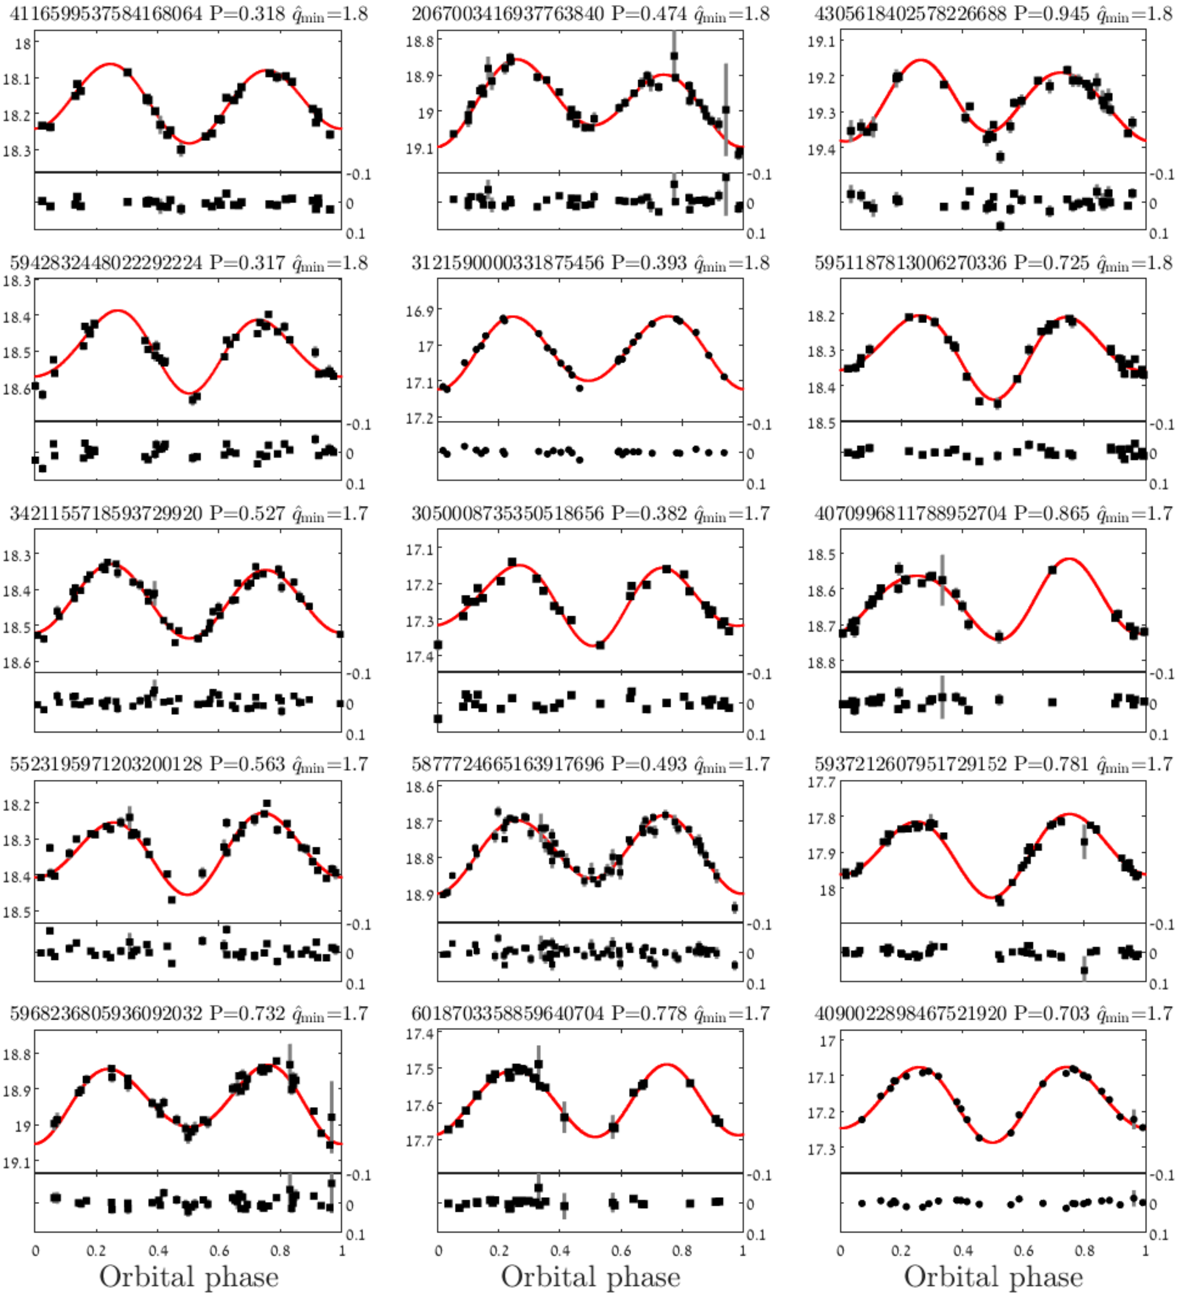


Fig. S1: Continued

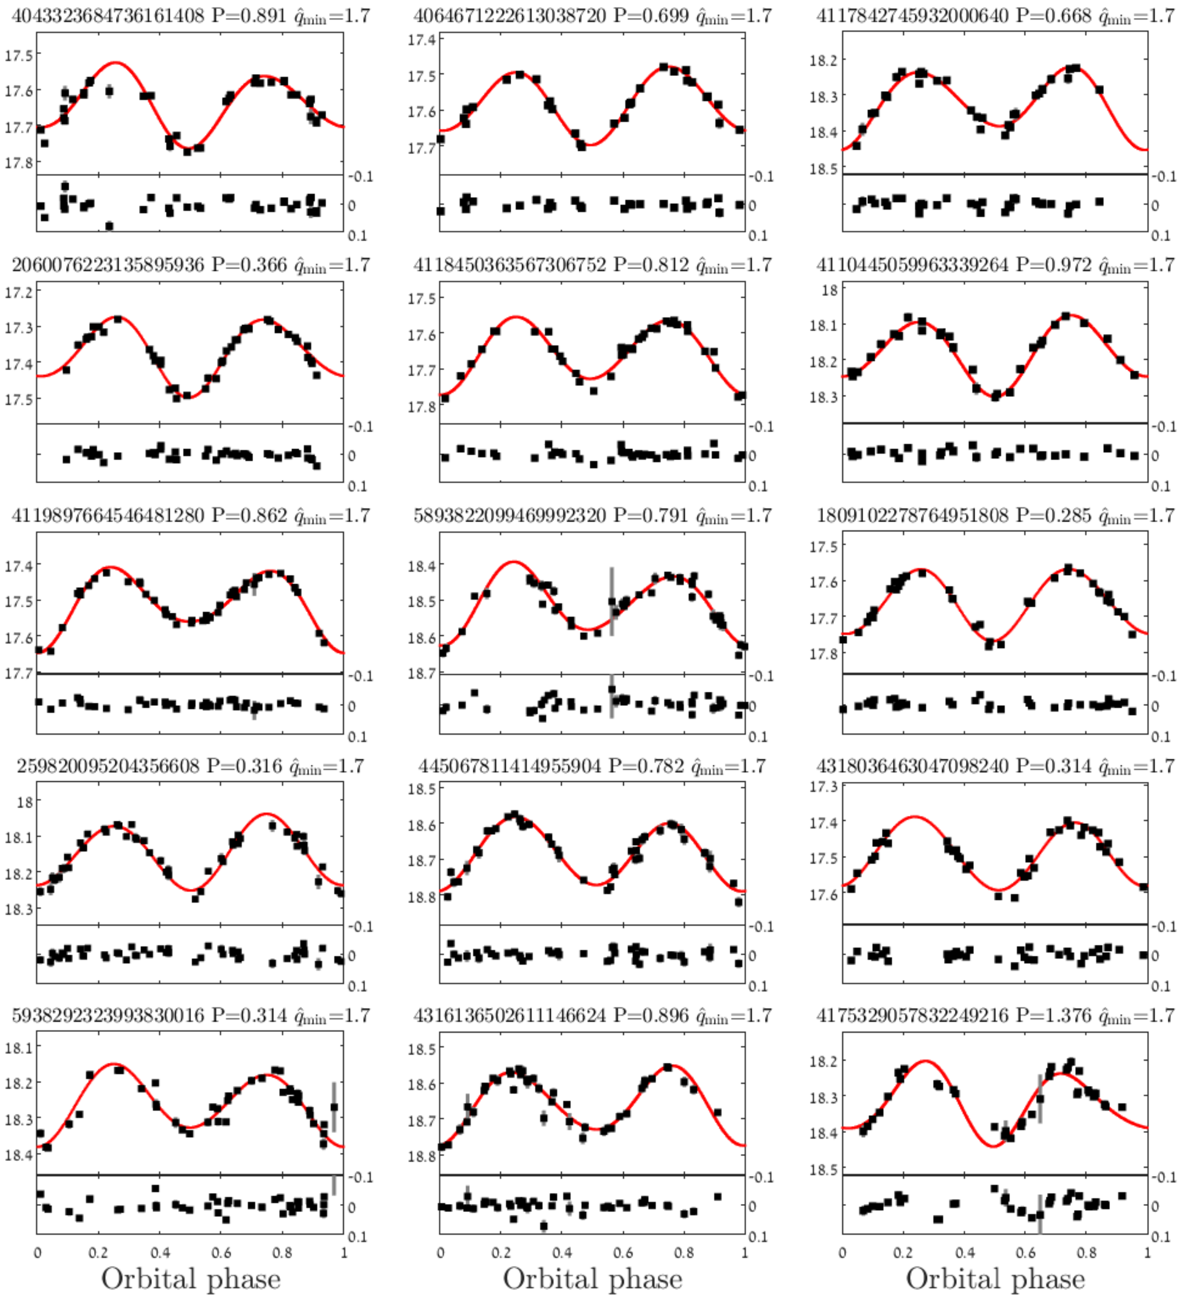


Fig. S1: Continued

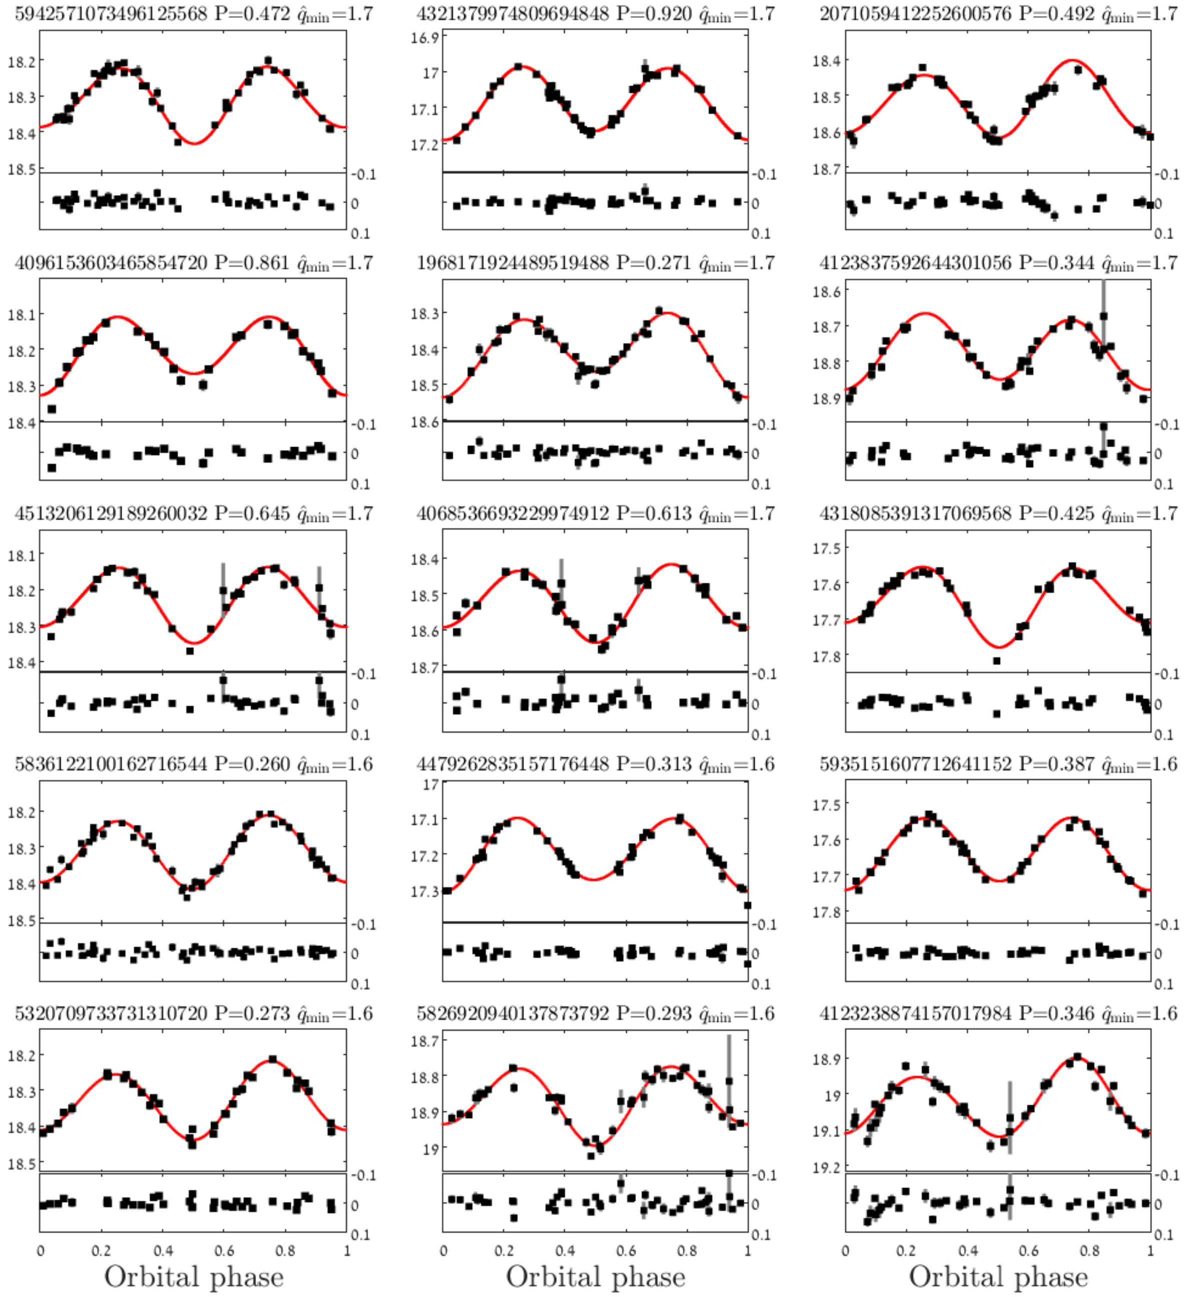


Fig. S1: Continued

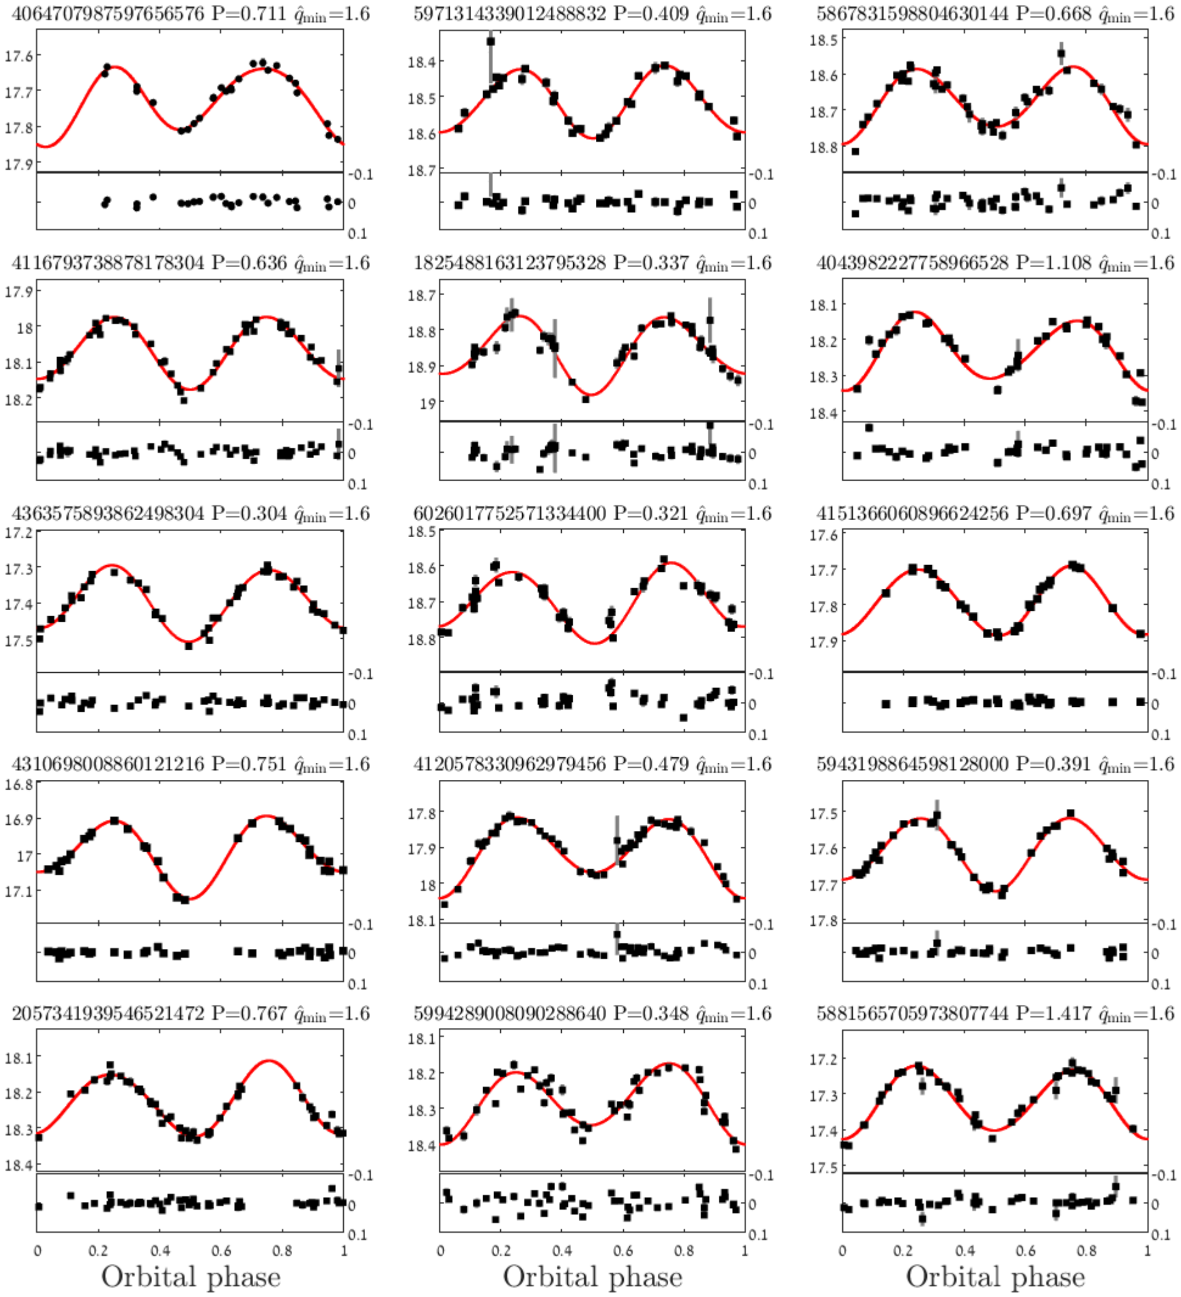


Fig. S1: Continued

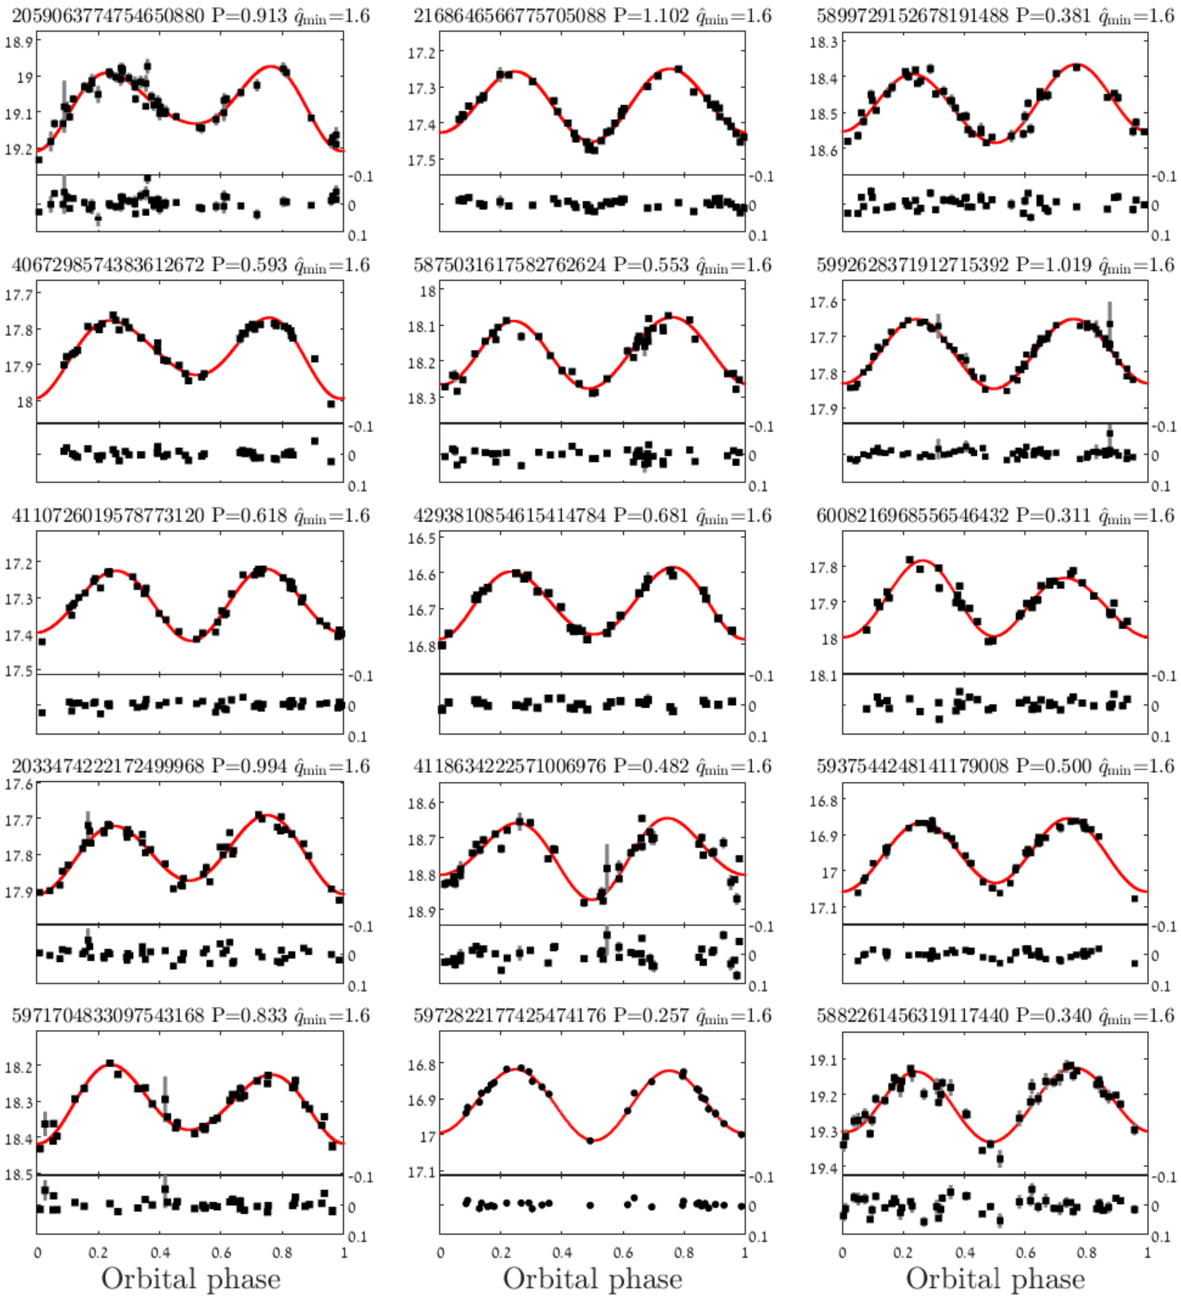


Fig. S1: Continued

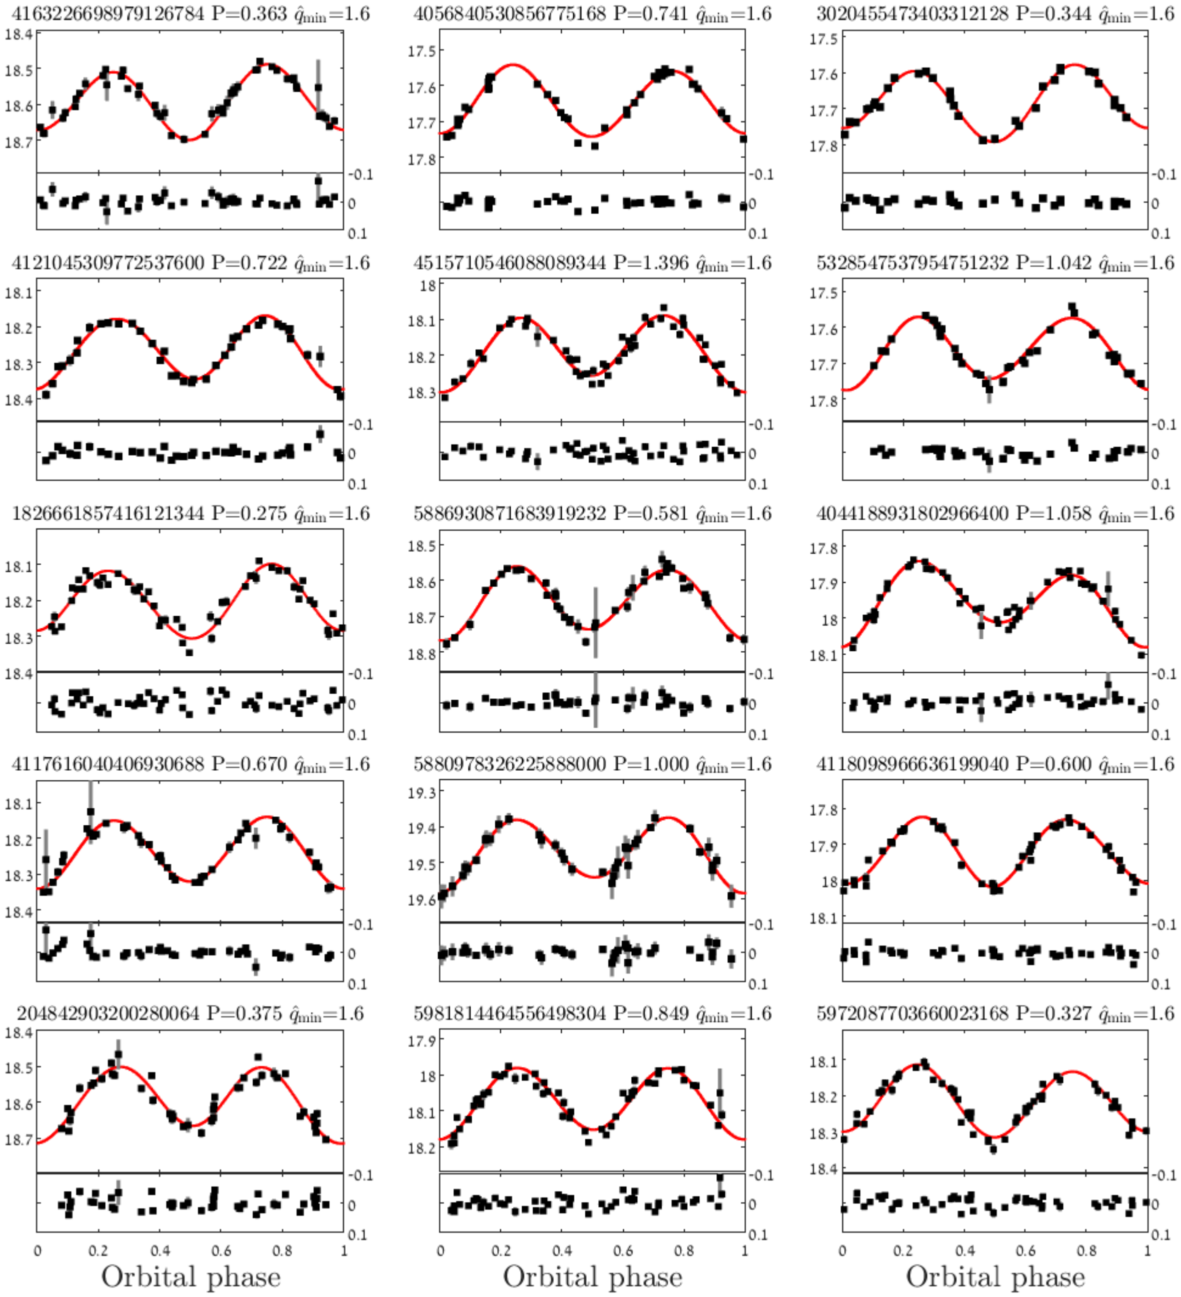


Fig. S1: Continued

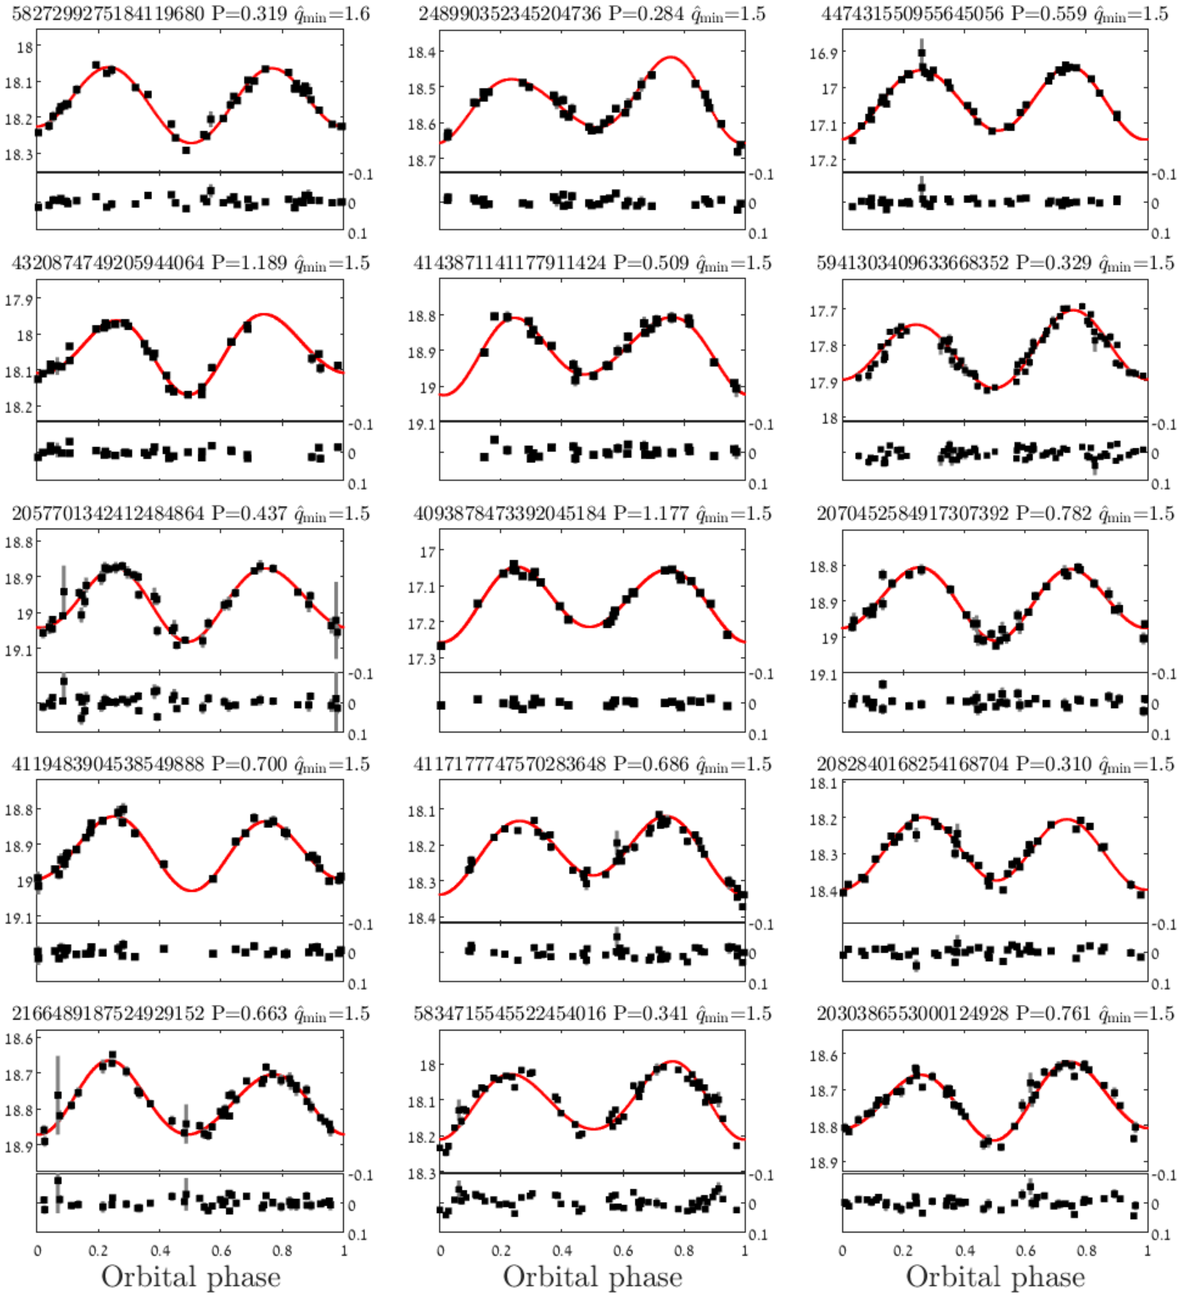


Fig. S1: Continued

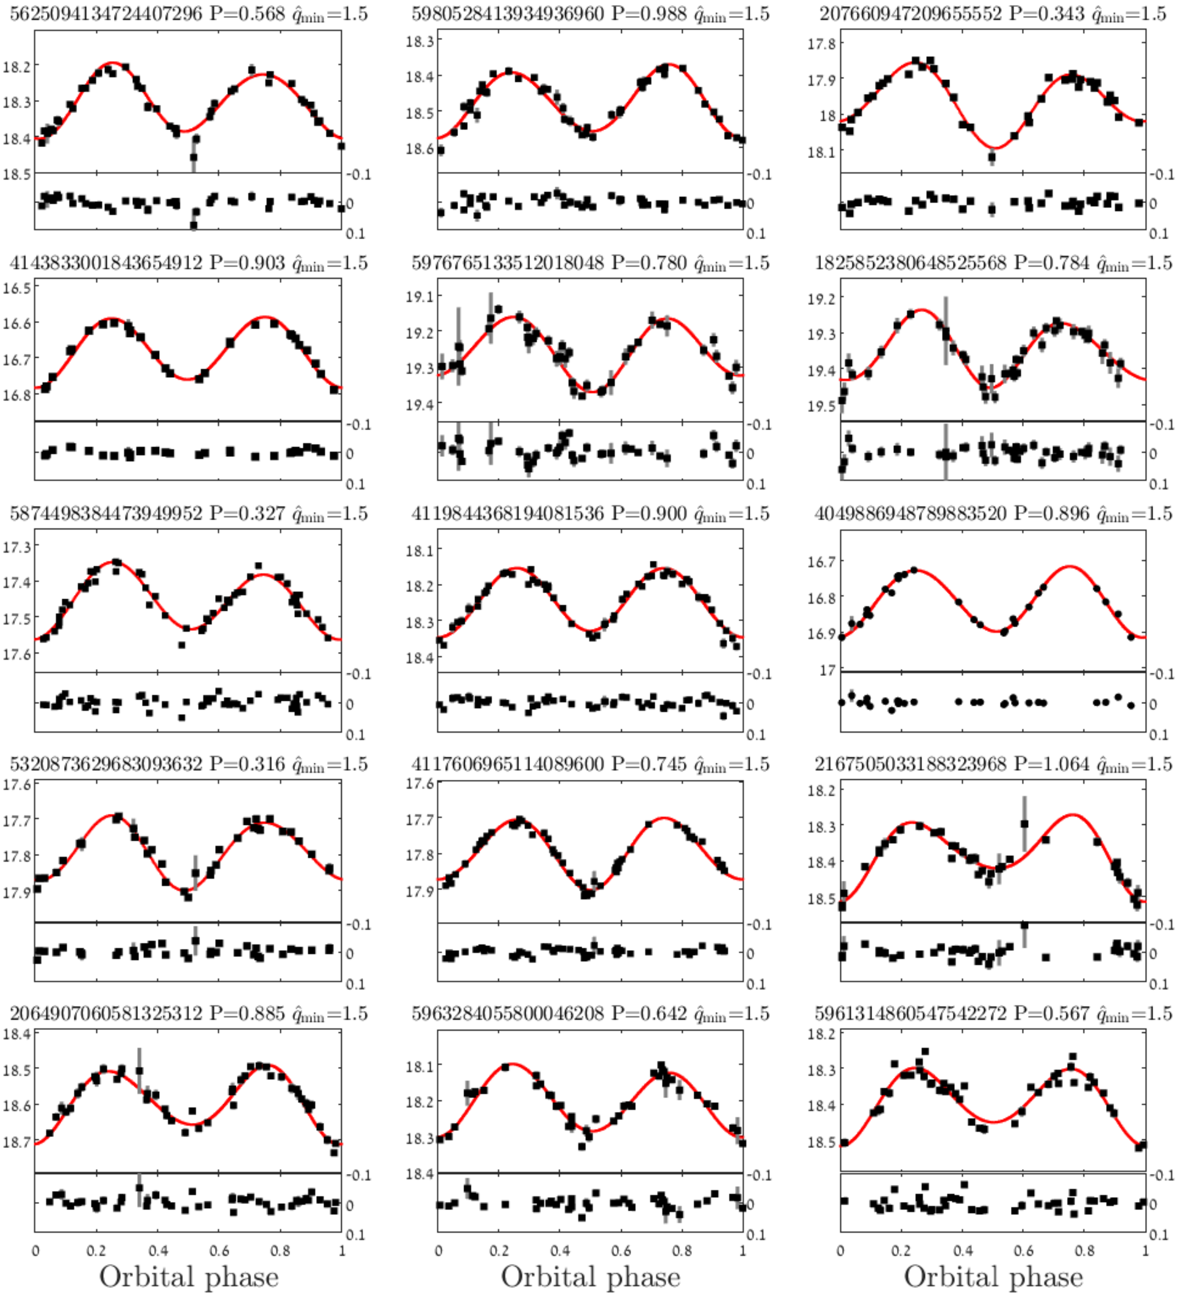


Fig. S1: Continued

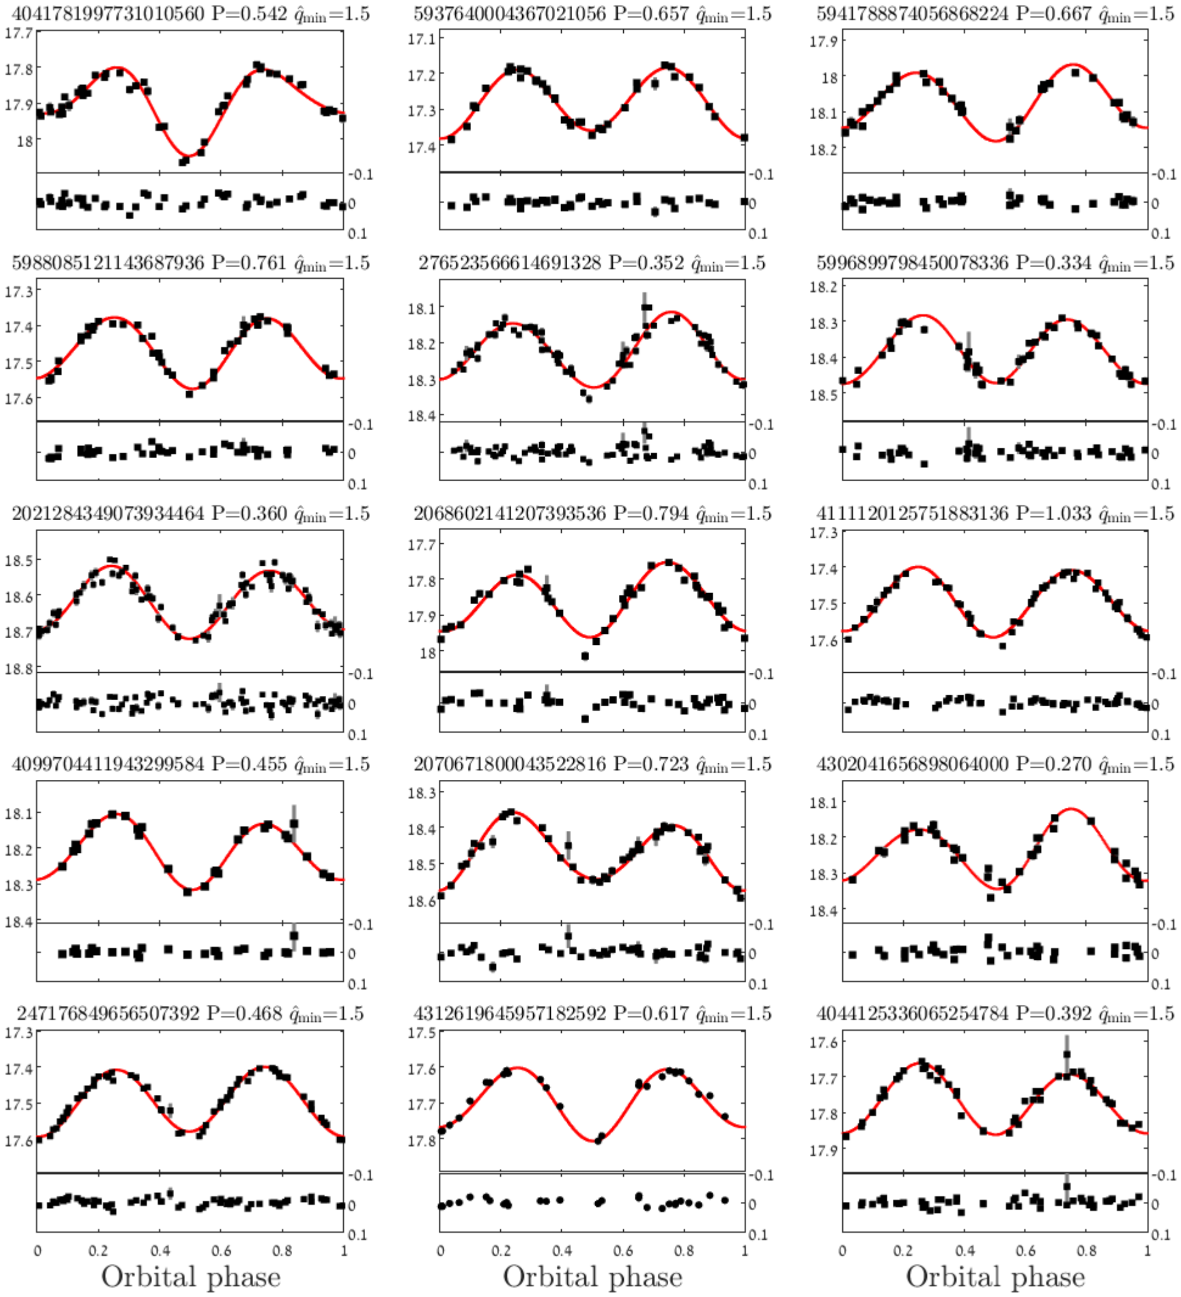


Fig. S1: Continued

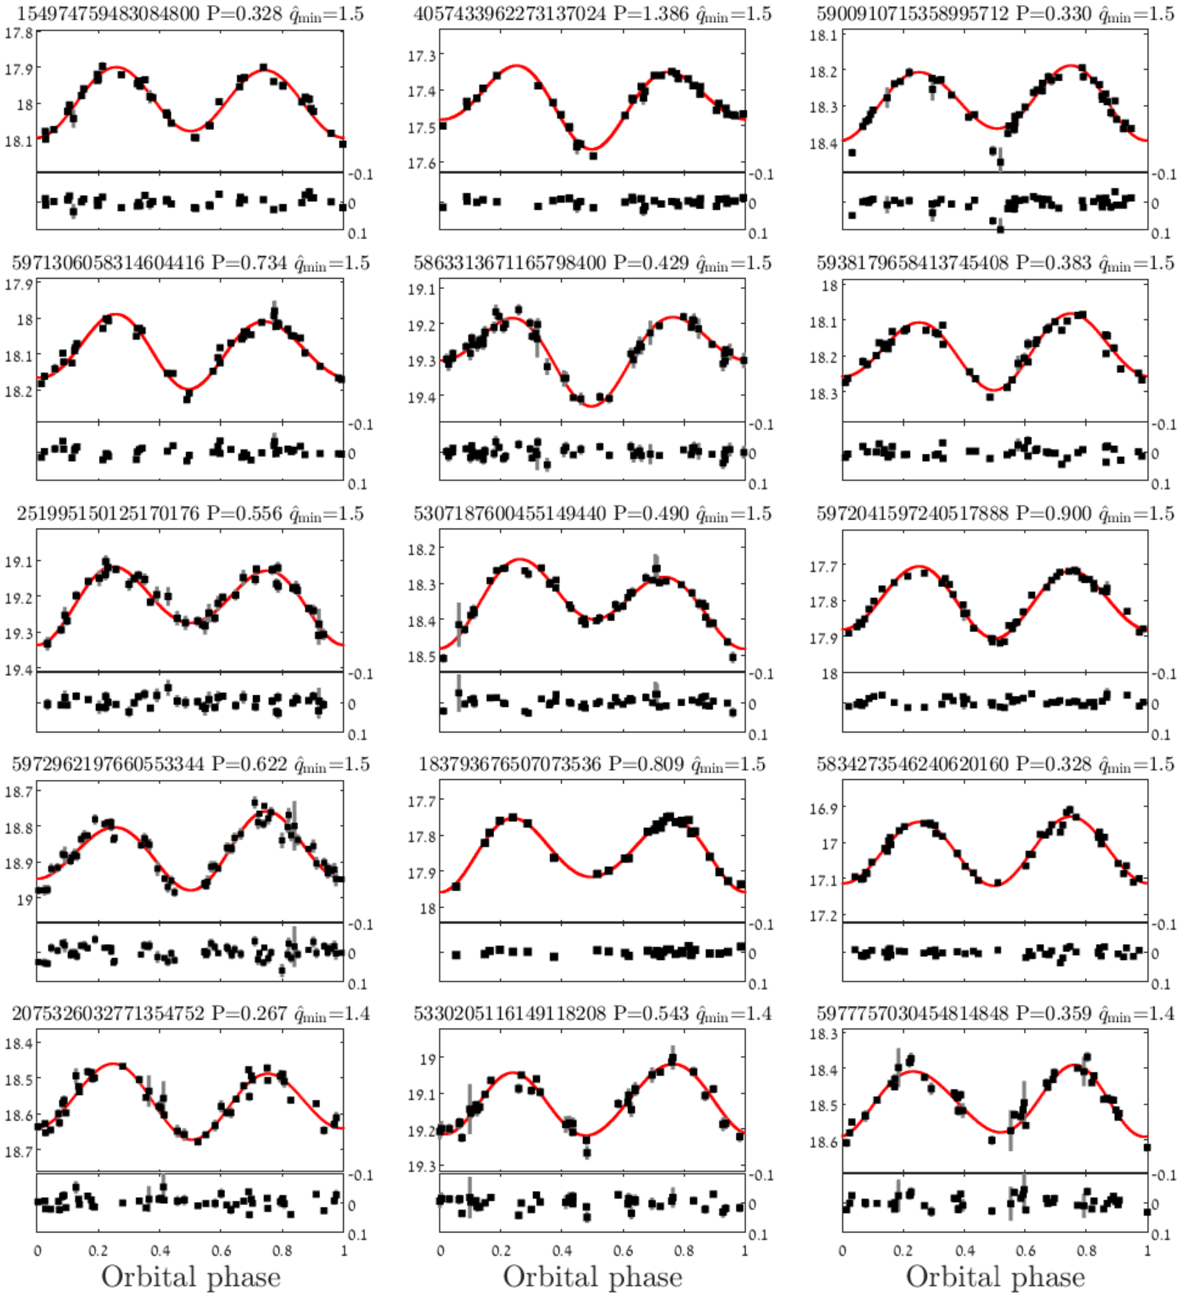


Fig. S1: Continued

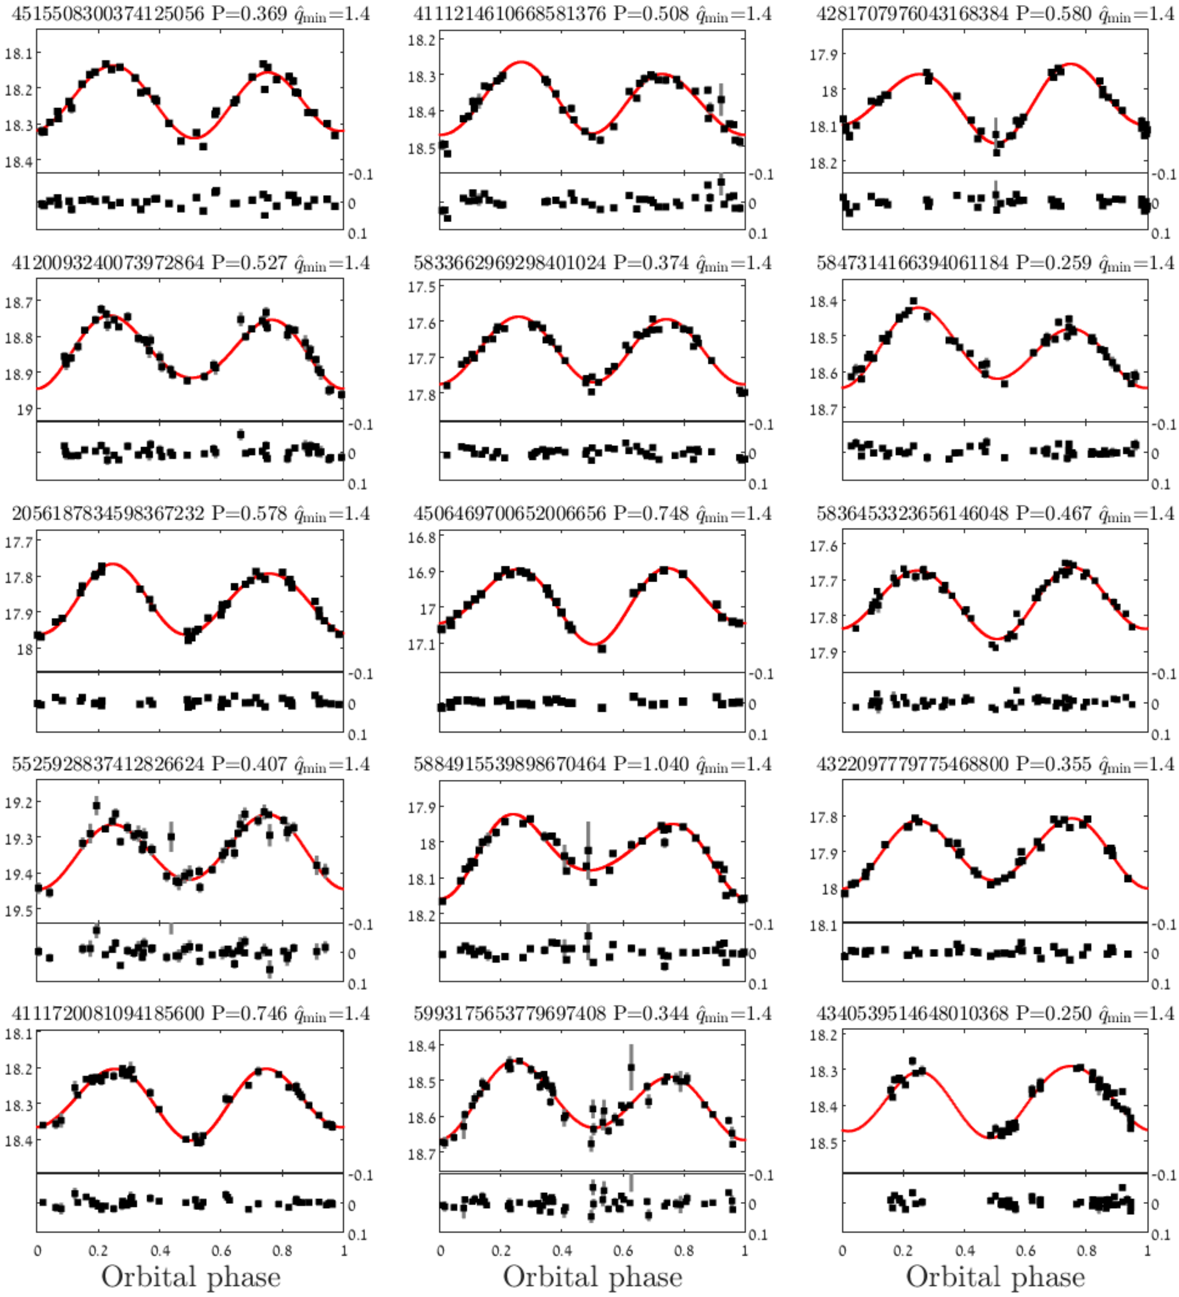


Fig. S1: Continued

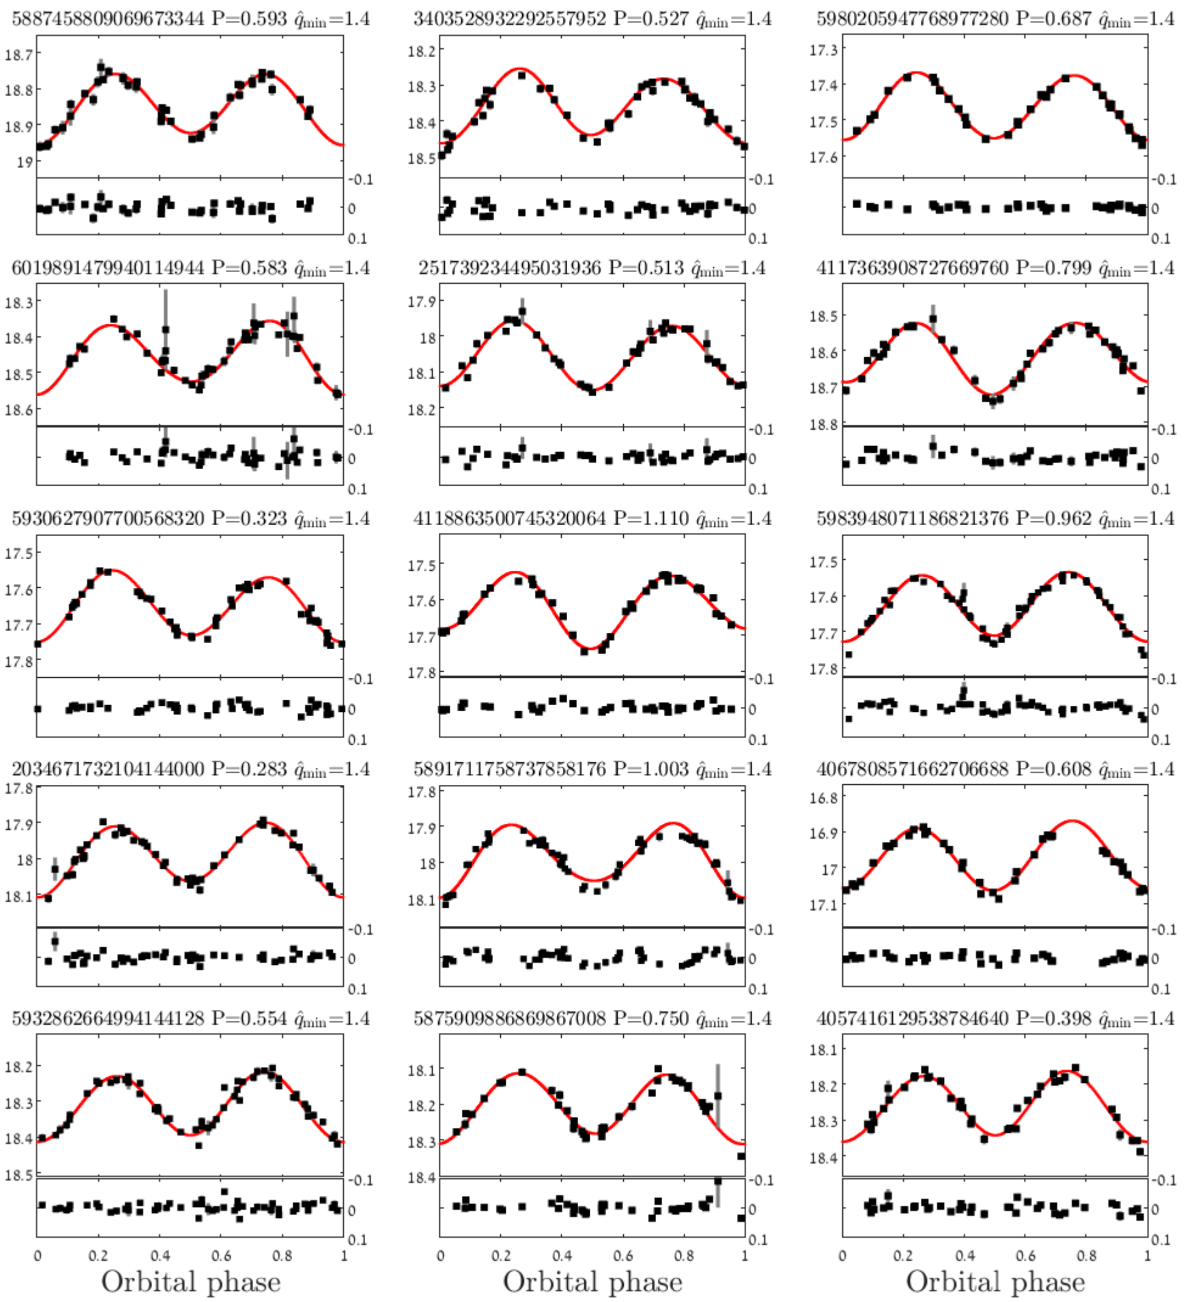


Fig. S1: Continued

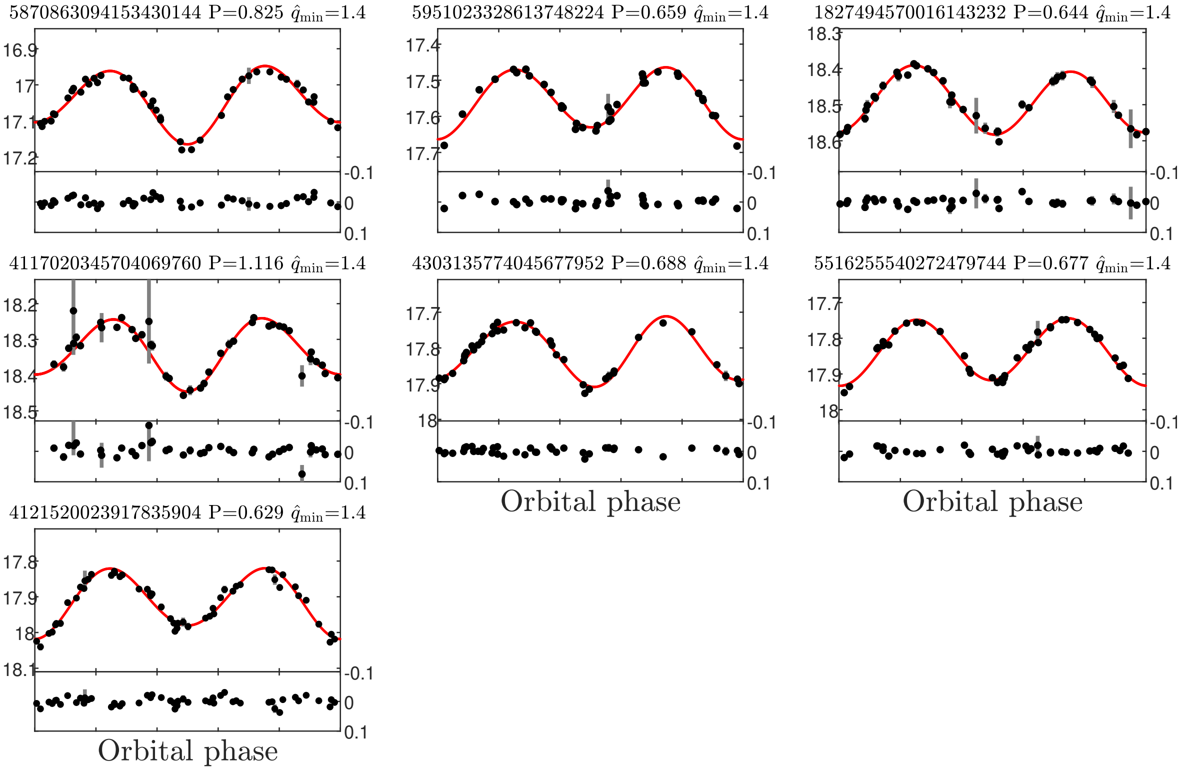


Fig. S1: Continued

| ***Gaia*** **DR3** | $P$ | $T_0$ | $\overline{G}$ | $a_{1c}$ | $a_{2c}$ | $a_{3c}$ | $a_{1s}$ | $a_{2s}$ | $a_{3s}$ | $N$ | $\hat{q}_{\rm min}$ | $\hat{q}_{\rm min}^{-1\sigma}$ |
|---|---|---|---|---|---|---|---|---|---|---|---|---|
| | $P_{\rm err}$ | $T_{0,\rm err}$ | $\overline{G}_{\rm err}$ | $a_{1c,\rm err}$ | $a_{2c,\rm err}$ | $a_{3c,\rm err}$ | $a_{1s,\rm err}$ | $a_{2s,\rm err}$ | $a_{3s,\rm err}$ | | | |
| | [day] | BJD − 2455197.5 | [mag] | [mag] | [mag] | [mag] | [mag] | [mag] | [mag] | | | |
| 5938420387082046976 | 0.314117 | 2244.03610 | 17.8719 | 0.0098 | 0.1315 | -0.0026 | 0.0226 | 0.0000 | -0.0115 | 43 | 10.0 | 5.6 |
| | 0.000054 | 0.00056 | 0.0018 | 0.0028 | 0.0036 | 0.0026 | 0.0033 | 0.0021 | 0.0035 | | | |
| 2613886138222158464 | 0.49774 | 2423.3476 | 18.6571 | -0.0103 | 0.1105 | 0.0229 | -0.0110 | 0.0000 | 0.0079 | 46 | 3.4 | 2.1 |
| | 0.00012 | 0.0020 | 0.0039 | 0.0047 | 0.0065 | 0.0067 | 0.0067 | 0.0046 | 0.0057 | | | |
| 4123054392395089920 | 0.62299 | 2425.4947 | 17.7272 | -0.0101 | 0.1104 | -0.0109 | 0.0220 | 0.0000 | -0.0105 | 43 | 3.4 | 2.2 |
| | 0.00021 | 0.0013 | 0.0031 | 0.0023 | 0.0047 | 0.0029 | 0.0055 | 0.0024 | 0.0038 | | | |
| 1892965058567426560 | 0.261008 | 2191.02880 | 17.6875 | 0.0023 | 0.1097 | 0.0008 | -0.0062 | 0.0000 | 0.0113 | 36 | 3.3 | 2.2 |
| | 0.000044 | 0.00049 | 0.0022 | 0.0033 | 0.0035 | 0.0028 | 0.0028 | 0.0026 | 0.0033 | | | |
| 4041883019496151424 | 1.12284 | 2355.7487 | 18.3060 | -0.0314 | 0.1097 | 0.0003 | -0.0068 | 0.0000 | 0.0041 | 34 | 3.3 | 2.1 |
| | 0.00077 | 0.0054 | 0.0036 | 0.0057 | 0.0061 | 0.0052 | 0.0055 | 0.0063 | 0.0054 | | | |
| 4116728150381233280 | 0.330273 | 2487.1291 | 18.7504 | 0.0175 | 0.1078 | 0.0123 | -0.0068 | 0.0000 | 0.0032 | 53 | 3.0 | 1.9 |
| | 0.000043 | 0.0014 | 0.0035 | 0.0059 | 0.0074 | 0.0061 | 0.0061 | 0.0040 | 0.0059 | | | |
| 6038453229081523072 | 0.327324 | 2105.02175 | 16.5562 | -0.0002 | 0.1073 | 0.0019 | -0.0101 | 0.0000 | 0.0057 | 41 | 2.9 | 2.0 |
| | 0.000082 | 0.00072 | 0.0020 | 0.0035 | 0.0042 | 0.0037 | 0.0033 | 0.0023 | 0.0031 | | | |
| 4516392793079294976 | 0.316059 | 2159.86061 | 18.9664 | 0.0214 | 0.1066 | 0.0048 | 0.0014 | 0.0000 | 0.0034 | 41 | 2.9 | 1.9 |
| | 0.000046 | 0.00074 | 0.0019 | 0.0032 | 0.0035 | 0.0029 | 0.0028 | 0.0026 | 0.0033 | | | |
| 4056017172771375616 | 0.410707 | 2394.25673 | 16.9046 | -0.0038 | 0.1066 | -0.0008 | -0.0049 | 0.0000 | 0.0112 | 44 | 2.9 | 1.9 |
| | 0.000093 | 0.00078 | 0.0016 | 0.0023 | 0.0031 | 0.0024 | 0.0027 | 0.0024 | 0.0028 | | | |
| 5889592931122816512 | 0.341463 | 2204.82654 | 18.3464 | 0.0162 | 0.1044 | -0.0004 | -0.0033 | 0.0000 | -0.0129 | 39 | 2.6 | 1.8 |
| | 0.000081 | 0.00084 | 0.0021 | 0.0031 | 0.0037 | 0.0030 | 0.0033 | 0.0026 | 0.0034 | | | |
| 4068402346632484864 | 1.27615 | 2356.9575 | 18.0847 | -0.0103 | 0.1043 | -0.0132 | -0.0015 | 0.0000 | 0.0135 | 39 | 2.6 | 1.6 |
| | 0.00079 | 0.0056 | 0.0044 | 0.0062 | 0.0070 | 0.0062 | 0.0064 | 0.0055 | 0.0061 | | | |
| 4042390512917208960 | 0.89522 | 2383.8996 | 13.7822 | 0.0000 | 0.1039 | -0.0074 | 0.0046 | 0.0000 | 0.0012 | 38 | 2.5 | 1.8 |
| | 0.00046 | 0.0014 | 0.0015 | 0.0022 | 0.0022 | 0.0023 | 0.0020 | 0.0020 | 0.0019 | | | |
| 1833609671396897024 | 1.20849 | 2202.2576 | 18.1657 | -0.0286 | 0.1035 | -0.0215 | -0.0010 | 0.0000 | -0.0083 | 53 | 2.5 | 1.7 |
| | 0.00074 | 0.0028 | 0.0028 | 0.0054 | 0.0048 | 0.0038 | 0.0030 | 0.0031 | 0.0038 | | | |
| 4068544041908031488 | 0.58456 | 2430.2668 | 18.9518 | 0.0258 | 0.1033 | 0.0116 | -0.0027 | 0.0000 | -0.0153 | 43 | 2.5 | 1.6 |
| | 0.00025 | 0.0026 | 0.0043 | 0.0063 | 0.0064 | 0.0064 | 0.0058 | 0.0057 | 0.0058 | | | |
| 6053386525470178560 | 0.96892 | 2206.1084 | 19.5447 | -0.0177 | 0.1032 | -0.0122 | 0.0016 | 0.0000 | -0.0040 | 40 | 2.5 | 1.6 |
| | 0.00052 | 0.0033 | 0.0035 | 0.0045 | 0.0055 | 0.0053 | 0.0053 | 0.0042 | 0.0047 | | | |

Table S1: Fitted parameters of the 262 candidates, in descending $\hat{q}_{\rm min}$ order.

| ***Gaia*** **DR3** | $P$ | $T_0$ | $\overline{G}$ | $a_{1c}$ | $a_{2c}$ | $a_{3c}$ | $a_{1s}$ | $a_{2s}$ | $a_{3s}$ | $N$ | $\hat{q}_{\rm min}$ | $\hat{q}_{\rm min}^{-1\sigma}$ |
|---|---|---|---|---|---|---|---|---|---|---|---|---|
| | $P_{\rm err}$ | $T_{0,\rm err}$ | $\overline{G}_{\rm err}$ | $a_{1c,\rm err}$ | $a_{2c,\rm err}$ | $a_{3c,\rm err}$ | $a_{1s,\rm err}$ | $a_{2s,\rm err}$ | $a_{3s,\rm err}$ | | | |
| | [day] | BJD − 2455197.5 | [mag] | [mag] | [mag] | [mag] | [mag] | [mag] | [mag] | | | |
| 227985355226451712 | 0.346954 | 2100.87566 | 17.6393 | -0.0127 | 0.1032 | 0.0012 | 0.0031 | 0.0000 | -0.0047 | 39 | 2.5 | 1.7 |
| | 0.000076 | 0.00066 | 0.0021 | 0.0036 | 0.0039 | 0.0030 | 0.0028 | 0.0024 | 0.0035 | | | |
| 4042492733124112640 | 0.97511 | 2350.6056 | 18.1594 | -0.0169 | 0.1025 | -0.0016 | -0.0144 | 0.0000 | 0.0039 | 34 | 2.4 | 1.6 |
| | 0.00056 | 0.0042 | 0.0043 | 0.0062 | 0.0056 | 0.0046 | 0.0049 | 0.0054 | 0.0065 | | | |
| 2034263023023544320 | 1.7873 | 2211.1771 | 18.6164 | 0.0277 | 0.1023 | 0.0105 | 0.0020 | 0.0000 | -0.0073 | 53 | 2.4 | 1.6 |
| | 0.0021 | 0.0055 | 0.0031 | 0.0040 | 0.0046 | 0.0035 | 0.0048 | 0.0041 | 0.0055 | | | |
| 4049067258553241216 | 1.19073 | 2290.2698 | 17.4659 | 0.0133 | 0.1017 | 0.0098 | -0.0008 | 0.0000 | 0.0025 | 29 | 2.3 | 1.5 |
| | 0.00079 | 0.0047 | 0.0044 | 0.0039 | 0.0064 | 0.0048 | 0.0085 | 0.0046 | 0.0068 | | | |
| 4383313295810461184 | 0.259789 | 2185.5570 | 17.9288 | 0.0013 | 0.1017 | -0.0082 | 0.0234 | 0.0000 | -0.0067 | 51 | 2.3 | 1.5 |
| | 0.000035 | 0.0011 | 0.0038 | 0.0033 | 0.0064 | 0.0047 | 0.0073 | 0.0039 | 0.0045 | | | |
| 5985264010492665216 | 0.264161 | 2103.22994 | 19.3656 | 0.0143 | 0.1011 | 0.0082 | 0.0080 | 0.0000 | 0.0030 | 48 | 2.2 | 1.5 |
| | 0.000047 | 0.00095 | 0.0032 | 0.0049 | 0.0049 | 0.0045 | 0.0042 | 0.0042 | 0.0045 | | | |
| 5939640634494621440 | 0.292932 | 2269.33105 | 17.9057 | -0.0190 | 0.1006 | -0.0076 | -0.0082 | 0.0000 | -0.0005 | 38 | 2.2 | 1.5 |
| | 0.000062 | 0.00082 | 0.0024 | 0.0041 | 0.0042 | 0.0033 | 0.0030 | 0.0028 | 0.0036 | | | |
| 2186314206807858048 | 0.273138 | 2214.85392 | 18.4732 | -0.0184 | 0.1003 | -0.0018 | -0.0215 | 0.0000 | 0.0033 | 36 | 2.2 | 1.5 |
| | 0.000054 | 0.00087 | 0.0029 | 0.0044 | 0.0050 | 0.0038 | 0.0043 | 0.0036 | 0.0045 | | | |
| 1824905460657943936 | 0.47632 | 2148.1579 | 18.4914 | -0.0025 | 0.1003 | -0.0150 | -0.0057 | 0.0000 | -0.0030 | 44 | 2.2 | 1.5 |
| | 0.00018 | 0.0016 | 0.0032 | 0.0043 | 0.0050 | 0.0040 | 0.0050 | 0.0042 | 0.0057 | | | |
| 5990533252504976896 | 0.92363 | 2164.5275 | 17.6908 | -0.0280 | 0.0999 | -0.0110 | 0.0115 | 0.0000 | 0.0049 | 42 | 2.1 | 1.5 |
| | 0.00049 | 0.0023 | 0.0023 | 0.0036 | 0.0036 | 0.0028 | 0.0027 | 0.0026 | 0.0032 | | | |
| 5942287781774326016 | 0.59140 | 2134.7088 | 19.1645 | -0.0153 | 0.0999 | 0.0017 | -0.0014 | 0.0000 | -0.0017 | 42 | 2.1 | 1.4 |
| | 0.00021 | 0.0024 | 0.0035 | 0.0046 | 0.0054 | 0.0050 | 0.0054 | 0.0046 | 0.0046 | | | |
| 4070409432055253760 | 0.64373 | 2251.7337 | 16.6490 | -0.0139 | 0.0995 | 0.0015 | 0.0005 | 0.0000 | 0.0045 | 29 | 2.1 | 1.5 |
| | 0.00027 | 0.0013 | 0.0018 | 0.0026 | 0.0027 | 0.0026 | 0.0025 | 0.0026 | 0.0028 | | | |
| 5887986922603177984 | 0.48350 | 2177.3829 | 17.5471 | -0.0124 | 0.0994 | -0.0036 | 0.0080 | 0.0000 | 0.0037 | 43 | 2.1 | 1.5 |
| | 0.00013 | 0.0011 | 0.0021 | 0.0036 | 0.0031 | 0.0031 | 0.0023 | 0.0026 | 0.0025 | | | |
| 4123554910705949184 | 0.46367 | 2410.1052 | 18.1393 | -0.0161 | 0.0993 | -0.0048 | -0.0025 | 0.0000 | -0.0012 | 43 | 2.1 | 1.4 |
| | 0.00014 | 0.0014 | 0.0026 | 0.0036 | 0.0042 | 0.0036 | 0.0038 | 0.0036 | 0.0041 | | | |
| 4049863167529174528 | 1.2326 | 2271.6591 | 17.7074 | 0.0006 | 0.0991 | -0.0020 | 0.0038 | 0.0000 | -0.0113 | 29 | 2.1 | 1.4 |
| | 0.0012 | 0.0045 | 0.0041 | 0.0043 | 0.0038 | 0.0041 | 0.0065 | 0.0054 | 0.0031 | | | |

Table S1: Continued.

| ***Gaia*** **DR3** | $P$ | $T_0$ | $\overline{G}$ | $a_{1c}$ | $a_{2c}$ | $a_{3c}$ | $a_{1s}$ | $a_{2s}$ | $a_{3s}$ | $N$ | $\hat{q}_{\rm min}$ | $\hat{q}_{\rm min}^{-1\sigma}$ |
|---|---|---|---|---|---|---|---|---|---|---|---|---|
| | $P_{\rm err}$ | $T_{0,\rm err}$ | $\overline{G}_{\rm err}$ | $a_{1c,\rm err}$ | $a_{2c,\rm err}$ | $a_{3c,\rm err}$ | $a_{1s,\rm err}$ | $a_{2s,\rm err}$ | $a_{3s,\rm err}$ | | | |
| | [day] | BJD − 2455197.5 | [mag] | [mag] | [mag] | [mag] | [mag] | [mag] | [mag] | | | |
| 4321356266589507584 | 0.302408 | 2129.1235 | 18.0994 | 0.0135 | 0.0990 | 0.0053 | -0.0045 | 0.0000 | 0.0100 | 40 | 2.1 | 1.4 |
| | 0.000060 | 0.0010 | 0.0033 | 0.0043 | 0.0053 | 0.0044 | 0.0054 | 0.0043 | 0.0054 | | | |
| 4111472617942868480 | 0.90575 | 2264.5219 | 17.5415 | -0.0288 | 0.0990 | -0.0089 | -0.0028 | 0.0000 | 0.0043 | 34 | 2.0 | 1.4 |
| | 0.00064 | 0.0036 | 0.0032 | 0.0050 | 0.0049 | 0.0041 | 0.0043 | 0.0044 | 0.0042 | | | |
| 4133786897189283840 | 0.323572 | 2232.55965 | 17.4026 | -0.0050 | 0.0990 | 0.0042 | -0.0102 | 0.0000 | 0.0029 | 54 | 2.0 | 1.4 |
| | 0.000083 | 0.00088 | 0.0022 | 0.0034 | 0.0038 | 0.0033 | 0.0032 | 0.0028 | 0.0032 | | | |
| 1811641429068979456 | 0.294163 | 2208.37283 | 17.1962 | -0.0113 | 0.0989 | 0.0008 | -0.0048 | 0.0000 | -0.0021 | 41 | 2.0 | 1.4 |
| | 0.000054 | 0.00087 | 0.0026 | 0.0033 | 0.0046 | 0.0032 | 0.0046 | 0.0031 | 0.0047 | | | |
| 4119752632040146816 | 0.54544 | 2378.5514 | 18.8840 | 0.0298 | 0.0989 | 0.0095 | -0.0179 | 0.0000 | -0.0086 | 41 | 2.0 | 1.3 |
| | 0.00020 | 0.0024 | 0.0049 | 0.0085 | 0.0071 | 0.0063 | 0.0047 | 0.0052 | 0.0060 | | | |
| 5978280432323971200 | 0.50856 | 2286.5397 | 18.4474 | -0.0075 | 0.0987 | -0.0141 | 0.0082 | 0.0000 | 0.0001 | 48 | 2.0 | 1.4 |
| | 0.00020 | 0.0020 | 0.0035 | 0.0056 | 0.0055 | 0.0047 | 0.0046 | 0.0045 | 0.0066 | | | |
| 6029163558415639936 | 0.283148 | 2314.48228 | 17.7682 | -0.0130 | 0.0986 | -0.0053 | -0.0082 | 0.0000 | -0.0008 | 42 | 2.0 | 1.4 |
| | 0.000046 | 0.00073 | 0.0023 | 0.0035 | 0.0042 | 0.0035 | 0.0035 | 0.0031 | 0.0035 | | | |
| 5929021035796328448 | 0.266586 | 2209.99661 | 18.6203 | -0.0222 | 0.0986 | -0.0063 | -0.0080 | 0.0000 | 0.0020 | 45 | 2.0 | 1.3 |
| | 0.000050 | 0.00098 | 0.0035 | 0.0056 | 0.0058 | 0.0051 | 0.0045 | 0.0040 | 0.0048 | | | |
| 3005724873744854400 | 0.353007 | 2212.0273 | 17.6909 | -0.0204 | 0.0985 | -0.0058 | 0.0128 | 0.0000 | -0.0030 | 31 | 2.0 | 1.3 |
| | 0.000064 | 0.0010 | 0.0031 | 0.0052 | 0.0056 | 0.0061 | 0.0046 | 0.0036 | 0.0044 | | | |
| 5532108401998093056 | 0.281160 | 2223.88025 | 17.5074 | 0.0153 | 0.0983 | -0.0023 | 0.0015 | 0.0000 | -0.0054 | 41 | 2.0 | 1.4 |
| | 0.000042 | 0.00066 | 0.0020 | 0.0028 | 0.0032 | 0.0030 | 0.0030 | 0.0026 | 0.0029 | | | |
| 1827765565254918272 | 0.96806 | 2184.8263 | 19.0914 | -0.0213 | 0.0981 | -0.0112 | 0.0066 | 0.0000 | -0.0160 | 44 | 2.0 | 1.2 |
| | 0.00067 | 0.0052 | 0.0048 | 0.0060 | 0.0083 | 0.0062 | 0.0081 | 0.0057 | 0.0073 | | | |
| 2072345669060000640 | 0.373967 | 2232.69385 | 17.6158 | -0.0141 | 0.0981 | 0.0000 | 0.0006 | 0.0000 | 0.0017 | 43 | 2.0 | 1.4 |
| | 0.000079 | 0.00072 | 0.0017 | 0.0023 | 0.0030 | 0.0023 | 0.0029 | 0.0023 | 0.0033 | | | |
| 4117344014362469248 | 1.12572 | 2384.9853 | 17.9077 | 0.0087 | 0.0980 | 0.0048 | -0.0001 | 0.0000 | -0.0039 | 42 | 2.0 | 1.4 |
| | 0.00058 | 0.0031 | 0.0021 | 0.0026 | 0.0035 | 0.0031 | 0.0034 | 0.0031 | 0.0034 | | | |
| 5938370526760023552 | 0.41678 | 2277.48949 | 17.8870 | -0.0150 | 0.0980 | 0.0030 | 0.0044 | 0.0000 | 0.0028 | 40 | 2.0 | 1.4 |
| | 0.00015 | 0.00087 | 0.0017 | 0.0026 | 0.0030 | 0.0032 | 0.0024 | 0.0025 | 0.0024 | | | |
| 4121502844048485120 | 1.09802 | 2406.0723 | 17.8135 | -0.0181 | 0.0979 | -0.0068 | -0.0032 | 0.0000 | -0.0029 | 51 | 2.0 | 1.4 |
| | 0.00076 | 0.0019 | 0.0015 | 0.0023 | 0.0022 | 0.0021 | 0.0021 | 0.0021 | 0.0020 | | | |

Table S1: Continued.

| ***Gaia*** **DR3** | $P$ | $T_0$ | $\overline{G}$ | $a_{1c}$ | $a_{2c}$ | $a_{3c}$ | $a_{1s}$ | $a_{2s}$ | $a_{3s}$ | $N$ | $\hat{q}_{\rm min}$ | $\hat{q}_{\rm min}^{-1\sigma}$ |
|---|---|---|---|---|---|---|---|---|---|---|---|---|
| | $P_{\rm err}$ | $T_{0,\rm err}$ | $\overline{G}_{\rm err}$ | $a_{1c,\rm err}$ | $a_{2c,\rm err}$ | $a_{3c,\rm err}$ | $a_{1s,\rm err}$ | $a_{2s,\rm err}$ | $a_{3s,\rm err}$ | | | |
| | [day] | BJD − 2455197.5 | [mag] | [mag] | [mag] | [mag] | [mag] | [mag] | [mag] | | | |
| 4059574436577349632 | 0.86396 | 2272.2939 | 16.9834 | 0.0063 | 0.0978 | -0.0011 | 0.0120 | 0.0000 | -0.0143 | 28 | 1.9 | 1.3 |
| | 0.00047 | 0.0027 | 0.0026 | 0.0037 | 0.0046 | 0.0036 | 0.0042 | 0.0031 | 0.0043 | | | |
| 2204247280119303808 | 0.319809 | 2226.6427 | 18.4264 | 0.0174 | 0.0978 | 0.0002 | -0.0032 | 0.0000 | -0.0023 | 33 | 1.9 | 1.3 |
| | 0.000072 | 0.0011 | 0.0030 | 0.0043 | 0.0047 | 0.0044 | 0.0039 | 0.0038 | 0.0043 | | | |
| 4315611283949759872 | 0.79238 | 2171.7412 | 19.2290 | -0.0180 | 0.0977 | -0.0164 | 0.0048 | 0.0000 | 0.0022 | 61 | 1.9 | 1.3 |
| | 0.00037 | 0.0027 | 0.0031 | 0.0043 | 0.0044 | 0.0044 | 0.0045 | 0.0044 | 0.0044 | | | |
| 5972653127516529024 | 0.44851 | 2219.8624 | 17.4636 | 0.0080 | 0.0976 | -0.0138 | 0.0009 | 0.0000 | -0.0009 | 28 | 1.9 | 1.4 |
| | 0.00021 | 0.0011 | 0.0023 | 0.0022 | 0.0034 | 0.0026 | 0.0041 | 0.0025 | 0.0031 | | | |
| 4107801593552947584 | 0.33705 | 2313.25335 | 17.4852 | -0.0140 | 0.0976 | 0.0039 | 0.0003 | 0.0000 | -0.0027 | 40 | 1.9 | 1.4 |
| | 0.00012 | 0.00080 | 0.0020 | 0.0027 | 0.0032 | 0.0027 | 0.0030 | 0.0026 | 0.0030 | | | |
| 4309230779322958080 | 1.4874 | 2197.3077 | 17.9579 | 0.0184 | 0.0976 | 0.0075 | -0.0104 | 0.0000 | 0.0014 | 30 | 1.9 | 1.3 |
| | 0.0015 | 0.0060 | 0.0035 | 0.0053 | 0.0052 | 0.0069 | 0.0046 | 0.0047 | 0.0040 | | | |
| 5889781870980547840 | 0.339736 | 2122.5855 | 18.4482 | -0.0217 | 0.0976 | 0.0045 | 0.0010 | 0.0000 | 0.0001 | 44 | 1.9 | 1.3 |
| | 0.000083 | 0.0010 | 0.0027 | 0.0047 | 0.0042 | 0.0037 | 0.0031 | 0.0032 | 0.0035 | | | |
| 5540344328205082880 | 0.305709 | 2238.7448 | 19.4390 | 0.0160 | 0.0974 | 0.0082 | 0.0023 | 0.0000 | 0.0019 | 50 | 1.9 | 1.3 |
| | 0.000061 | 0.0011 | 0.0033 | 0.0046 | 0.0056 | 0.0051 | 0.0050 | 0.0040 | 0.0046 | | | |
| 4361779429301138560 | 0.321689 | 2338.22731 | 17.9390 | 0.0109 | 0.0974 | 0.0149 | 0.0052 | 0.0000 | -0.0119 | 46 | 1.9 | 1.3 |
| | 0.000049 | 0.00078 | 0.0026 | 0.0045 | 0.0054 | 0.0042 | 0.0041 | 0.0029 | 0.0042 | | | |
| 5881690427478435584 | 0.54635 | 2165.2419 | 18.1461 | -0.0062 | 0.0974 | -0.0153 | -0.0119 | 0.0000 | 0.0019 | 43 | 1.9 | 1.3 |
| | 0.00018 | 0.0022 | 0.0035 | 0.0040 | 0.0048 | 0.0048 | 0.0054 | 0.0046 | 0.0045 | | | |
| 5934239528450798720 | 0.338507 | 2173.9736 | 18.7905 | 0.0233 | 0.0974 | -0.0052 | 0.0041 | 0.0000 | -0.0044 | 49 | 1.9 | 1.3 |
| | 0.000082 | 0.0014 | 0.0035 | 0.0050 | 0.0055 | 0.0051 | 0.0051 | 0.0046 | 0.0050 | | | |
| 5970830893156863104 | 0.95753 | 2268.9040 | 17.4940 | -0.0378 | 0.0974 | -0.0105 | 0.0041 | 0.0000 | -0.0011 | 44 | 1.9 | 1.3 |
| | 0.00065 | 0.0027 | 0.0024 | 0.0038 | 0.0040 | 0.0033 | 0.0032 | 0.0029 | 0.0037 | | | |
| 2055977827881625984 | 1.8189 | 2208.2701 | 18.1518 | 0.0086 | 0.0973 | 0.0069 | 0.043 | 0.0000 | -0.0194 | 49 | 1.9 | 1.2 |
| | 0.0025 | 0.0054 | 0.0056 | 0.0034 | 0.0086 | 0.0036 | 0.011 | 0.0039 | 0.0056 | | | |
| 5832556693145324800 | 0.355998 | 2177.88203 | 17.9045 | -0.0091 | 0.0970 | -0.0047 | -0.0024 | 0.0000 | 0.0060 | 46 | 1.9 | 1.3 |
| | 0.000084 | 0.00083 | 0.0021 | 0.0026 | 0.0034 | 0.0029 | 0.0034 | 0.0025 | 0.0033 | | | |
| 5977824543018395904 | 1.2407 | 2268.3179 | 17.4311 | -0.0092 | 0.0967 | -0.0107 | 0.0051 | 0.0000 | -0.0023 | 46 | 1.9 | 1.3 |
| | 0.0011 | 0.0033 | 0.0024 | 0.0029 | 0.0032 | 0.0030 | 0.0035 | 0.0031 | 0.0035 | | | |

Table S1: Continued.

| ***Gaia*** **DR3** | $P$ <br> $P_{err}$ <br> [day] | $T_0$ <br> $T_{0,err}$ <br> BJD − 2455197.5 | $\overline{G}$ <br> $\overline{G}_{err}$ <br> [mag] | $a_{1c}$ <br> $a_{1c,err}$ <br> [mag] | $a_{2c}$ <br> $a_{2c,err}$ <br> [mag] | $a_{3c}$ <br> $a_{3c,err}$ <br> [mag] | $a_{1s}$ <br> $a_{1s,err}$ <br> [mag] | $a_{2s}$ <br> $a_{2s,err}$ <br> [mag] | $a_{3s}$ <br> $a_{3s,err}$ <br> [mag] | $N$ | $\hat{q}_{min}$ | $\hat{q}_{min}^{-1\sigma}$ |
|---|---|---|---|---|---|---|---|---|---|---|---|---|
| 5962408672771256960 | 0.80764 <br> 0.00032 | 2444.4403 <br> 0.0036 | 19.1682 <br> 0.0038 | 0.0086 <br> 0.0059 | 0.0967 <br> 0.0056 | -0.0161 <br> 0.0055 | 0.0084 <br> 0.0049 | 0.0000 <br> 0.0051 | 0.0066 <br> 0.0049 | 49 | 1.9 | 1.3 |
| 2018326662796791808 | 0.259352 <br> 0.000044 | 2157.8739 <br> 0.0014 | 18.2798 <br> 0.0041 | -0.0207 <br> 0.0064 | 0.0966 <br> 0.0072 | -0.0011 <br> 0.0068 | 0.0273 <br> 0.0062 | 0.0000 <br> 0.0053 | -0.0070 <br> 0.0057 | 43 | 1.8 | 1.2 |
| 595231762993l188864 | 0.334504 <br> 0.000097 | 2209.82226 <br> 0.00063 | 17.7633 <br> 0.0019 | -0.0208 <br> 0.0033 | 0.0965 <br> 0.0039 | -0.0039 <br> 0.0035 | 0.0072 <br> 0.0030 | 0.0000 <br> 0.0023 | -0.0017 <br> 0.0029 | 43 | 1.8 | 1.3 |
| 3031142245391867008 | 0.87796 <br> 0.00044 | 2145.8138 <br> 0.0018 | 17.7199 <br> 0.0018 | -0.0014 <br> 0.0028 | 0.0965 <br> 0.0027 | 0.0020 <br> 0.0027 | -0.0001 <br> 0.0023 | 0.0000 <br> 0.0023 | -0.0076 <br> 0.0023 | 42 | 1.8 | 1.3 |
| 2062815793766426368 | 0.86602 <br> 0.00039 | 2231.7284 <br> 0.0019 | 17.8037 <br> 0.0020 | -0.0091 <br> 0.0029 | 0.0964 <br> 0.0031 | -0.0040 <br> 0.0027 | -0.0014 <br> 0.0027 | 0.0000 <br> 0.0026 | 0.0007 <br> 0.0029 | 59 | 1.8 | 1.3 |
| 4116865658058002176 | 0.66849 <br> 0.00027 | 2394.2923 <br> 0.0028 | 18.8996 <br> 0.0042 | 0.0264 <br> 0.0062 | 0.0964 <br> 0.0061 | 0.0115 <br> 0.0054 | -0.0027 <br> 0.0050 | 0.0000 <br> 0.0052 | 0.0109 <br> 0.0058 | 42 | 1.8 | 1.2 |
| 5887979226016445696 | 0.383677 <br> 0.000078 | 2157.62539 <br> 0.00082 | 17.8236 <br> 0.0020 | -0.0120 <br> 0.0029 | 0.0963 <br> 0.0032 | -0.0000 <br> 0.0027 | 0.0049 <br> 0.0030 | 0.0000 <br> 0.0026 | -0.0040 <br> 0.0031 | 50 | 1.8 | 1.3 |
| 4059248427022016128 | 0.95497 <br> 0.00057 | 2326.6792 <br> 0.0018 | 18.3441 <br> 0.0018 | 0.0084 <br> 0.0025 | 0.0963 <br> 0.0028 | 0.0021 <br> 0.0023 | 0.0013 <br> 0.0026 | 0.0000 <br> 0.0023 | 0.0011 <br> 0.0027 | 60 | 1.8 | 1.3 |
| 4322206498284428032 | 0.377082 <br> 0.000082 | 2144.2519 <br> 0.0015 | 19.0042 <br> 0.0034 | 0.0197 <br> 0.0053 | 0.0962 <br> 0.0053 | 0.0004 <br> 0.0057 | -0.0127 <br> 0.0049 | 0.0000 <br> 0.0046 | -0.0041 <br> 0.0058 | 39 | 1.8 | 1.2 |
| 6020259988135198080 | 1.1549 <br> 0.0010 | 2131.7325 <br> 0.0036 | 17.9963 <br> 0.0025 | 0.0243 <br> 0.0030 | 0.0961 <br> 0.0037 | 0.0132 <br> 0.0037 | -0.0059 <br> 0.0041 | 0.0000 <br> 0.0034 | -0.0008 <br> 0.0033 | 30 | 1.8 | 1.3 |
| 4141860374856674816 | 0.340986 <br> 0.000072 | 2335.1687 <br> 0.0012 | 17.7516 <br> 0.0026 | -0.0049 <br> 0.0039 | 0.0960 <br> 0.0048 | -0.0007 <br> 0.0037 | 0.0131 <br> 0.0041 | 0.0000 <br> 0.0032 | -0.0005 <br> 0.0042 | 47 | 1.8 | 1.2 |
| 5966221774764182272 | 0.37291 <br> 0.00010 | 2265.2092 <br> 0.0013 | 18.6073 <br> 0.0028 | 0.0125 <br> 0.0041 | 0.0960 <br> 0.0046 | -0.0080 <br> 0.0046 | -0.0008 <br> 0.0038 | 0.0000 <br> 0.0037 | -0.0006 <br> 0.0038 | 42 | 1.8 | 1.2 |
| 4117139329111282176 | 0.76374 <br> 0.00041 | 2417.3261 <br> 0.0022 | 18.9662 <br> 0.0027 | -0.0108 <br> 0.0043 | 0.0959 <br> 0.0037 | -0.0057 <br> 0.0035 | -0.0065 <br> 0.0032 | 0.0000 <br> 0.0035 | -0.0002 <br> 0.0038 | 41 | 1.8 | 1.3 |
| 2163883040038422272 | 0.350006 <br> 0.000066 | 2197.55162 <br> 0.00086 | 17.0853 <br> 0.0022 | 0.0039 <br> 0.0029 | 0.0958 <br> 0.0036 | 0.0003 <br> 0.0035 | -0.0103 <br> 0.0032 | 0.0000 <br> 0.0029 | 0.0020 <br> 0.0031 | 41 | 1.8 | 1.3 |
| 4123887787851678208 | 1.9493 <br> 0.0017 | 2422.9896 <br> 0.0069 | 18.0462 <br> 0.0032 | 0.0269 <br> 0.0046 | 0.0958 <br> 0.0045 | 0.0121 <br> 0.0039 | -0.0049 <br> 0.0040 | 0.0000 <br> 0.0043 | -0.0053 <br> 0.0046 | 60 | 1.8 | 1.2 |

Table S1: Continued.

| ***Gaia*** **DR3** | $P$<br>$P_{\rm err}$<br>[day] | $T_0$<br>$T_{0,\rm err}$<br>BJD − 2455197.5 | $\overline{G}$<br>$\overline{G}_{\rm err}$<br>[mag] | $a_{1c}$<br>$a_{1c,\rm err}$<br>[mag] | $a_{2c}$<br>$a_{2c,\rm err}$<br>[mag] | $a_{3c}$<br>$a_{3c,\rm err}$<br>[mag] | $a_{1s}$<br>$a_{1s,\rm err}$<br>[mag] | $a_{2s}$<br>$a_{2s,\rm err}$<br>[mag] | $a_{3s}$<br>$a_{3s,\rm err}$<br>[mag] | $N$ | $\hat{q}_{\rm min}$ | $\hat{q}_{\rm min}^{-1\sigma}$ |
|---|---|---|---|---|---|---|---|---|---|---|---|---|
| 4116599537584168064 | 0.318284 | 2263.99036 | 18.1669 | -0.0184 | 0.0957 | -0.0021 | -0.0082 | 0.0000 | 0.0006 | 31 | 1.8 | 1.3 |
| | 0.000058 | 0.00079 | 0.0025 | 0.0029 | 0.0040 | 0.0032 | 0.0042 | 0.0029 | 0.0037 | | | |
| 2067003416937763840 | 0.47401 | 2225.8240 | 18.9732 | 0.0280 | 0.0957 | 0.0022 | -0.0200 | 0.0000 | 0.0013 | 42 | 1.8 | 1.3 |
| | 0.00015 | 0.0012 | 0.0024 | 0.0032 | 0.0037 | 0.0031 | 0.0036 | 0.0031 | 0.0038 | | | |
| 4305618402578226688 | 0.94493 | 2154.3442 | 19.2713 | 0.0208 | 0.0956 | -0.0078 | -0.0042 | 0.0000 | 0.0143 | 33 | 1.8 | 1.2 |
| | 0.00066 | 0.0048 | 0.0045 | 0.0058 | 0.0064 | 0.0059 | 0.0065 | 0.0058 | 0.0062 | | | |
| 5942832448022292224 | 0.317324 | 2278.7801 | 18.4988 | -0.0044 | 0.0956 | -0.0192 | -0.0126 | 0.0000 | 0.0006 | 41 | 1.8 | 1.2 |
| | 0.000082 | 0.0013 | 0.0031 | 0.0045 | 0.0056 | 0.0047 | 0.0046 | 0.0052 | 0.0058 | | | |
| 3121590000331875456 | 0.39342 | 2255.81446 | 17.0162 | 0.0063 | 0.0954 | 0.0056 | 0.0039 | 0.0000 | 0.0034 | 27 | 1.8 | 1.3 |
| | 0.00010 | 0.00072 | 0.0014 | 0.0021 | 0.0025 | 0.0024 | 0.0020 | 0.0019 | 0.0021 | | | |
| 5951187813006270336 | 0.72532 | 2223.4078 | 18.3023 | -0.0249 | 0.0953 | -0.0162 | -0.0058 | 0.0000 | -0.0035 | 35 | 1.8 | 1.2 |
| | 0.00043 | 0.0023 | 0.0031 | 0.0040 | 0.0038 | 0.0045 | 0.0034 | 0.0036 | 0.0033 | | | |
| 3421155718593729920 | 0.52675 | 2329.3188 | 18.4338 | -0.0071 | 0.0953 | -0.0007 | -0.0080 | 0.0000 | 0.0003 | 50 | 1.7 | 1.2 |
| | 0.00022 | 0.0015 | 0.0025 | 0.0038 | 0.0036 | 0.0034 | 0.0032 | 0.0033 | 0.0034 | | | |
| 3050008735350518656 | 0.38212 | 2152.5508 | 17.2505 | -0.0117 | 0.0952 | -0.0166 | -0.0091 | 0.0000 | -0.0058 | 28 | 1.7 | 1.2 |
| | 0.00010 | 0.0014 | 0.0032 | 0.0039 | 0.0047 | 0.0050 | 0.0050 | 0.0043 | 0.0041 | | | |
| 4070996811788952704 | 0.86546 | 2276.3766 | 18.6344 | -0.0068 | 0.0950 | -0.0022 | 0.0042 | 0.0000 | -0.0197 | 30 | 1.7 | 1.1 |
| | 0.00060 | 0.0044 | 0.0044 | 0.0074 | 0.0071 | 0.0040 | 0.0058 | 0.0068 | 0.0060 | | | |
| 5523195971203200128 | 0.56308 | 2224.4810 | 18.3370 | -0.0143 | 0.0950 | -0.0101 | 0.0123 | 0.0000 | -0.0010 | 41 | 1.7 | 1.2 |
| | 0.00024 | 0.0026 | 0.0039 | 0.0061 | 0.0060 | 0.0056 | 0.0047 | 0.0050 | 0.0051 | | | |
| 5877724665163917696 | 0.49266 | 2264.5120 | 18.7859 | 0.0202 | 0.0950 | 0.0010 | 0.0027 | 0.0000 | -0.0046 | 64 | 1.7 | 1.2 |
| | 0.00016 | 0.0013 | 0.0023 | 0.0031 | 0.0035 | 0.0034 | 0.0034 | 0.0031 | 0.0036 | | | |
| 5937212607951729152 | 0.78141 | 2172.2278 | 17.8986 | -0.0251 | 0.0950 | -0.0074 | 0.0117 | 0.0000 | 0.0010 | 47 | 1.7 | 1.2 |
| | 0.00040 | 0.0017 | 0.0023 | 0.0034 | 0.0028 | 0.0023 | 0.0025 | 0.0029 | 0.0033 | | | |
| 5968236805936092032 | 0.73218 | 2235.3131 | 18.9345 | 0.0112 | 0.0950 | 0.0122 | 0.0018 | 0.0000 | -0.0039 | 42 | 1.7 | 1.2 |
| | 0.00047 | 0.0025 | 0.0027 | 0.0042 | 0.0038 | 0.0038 | 0.0035 | 0.0039 | 0.0038 | | | |
| 6018703358859640704 | 0.77763 | 2188.8142 | 17.5937 | -0.0018 | 0.0949 | -0.0007 | -0.0036 | 0.0000 | -0.0115 | 30 | 1.7 | 1.2 |
| | 0.00053 | 0.0025 | 0.0029 | 0.0054 | 0.0047 | 0.0033 | 0.0027 | 0.0027 | 0.0033 | | | |
| 4090022898467521920 | 0.70299 | 2212.5637 | 17.1720 | -0.0108 | 0.0949 | -0.0094 | 0.0013 | 0.0000 | 0.0009 | 26 | 1.7 | 1.2 |
| | 0.00040 | 0.0013 | 0.0017 | 0.0024 | 0.0022 | 0.0024 | 0.0021 | 0.0023 | 0.0021 | | | |

Table S1: Continued.

| ***Gaia*** **DR3** | $P$ | $T_0$ | $\overline{G}$ | $a_{1c}$ | $a_{2c}$ | $a_{3c}$ | $a_{1s}$ | $a_{2s}$ | $a_{3s}$ | $N$ | $\hat{q}_{\min}$ | $\hat{q}_{\min}^{-1\sigma}$ |
|---|---|---|---|---|---|---|---|---|---|---|---|---|
| | $P_{\rm err}$ | $T_{0,\rm err}$ | $\overline{G}_{\rm err}$ | $a_{1c,\rm err}$ | $a_{2c,\rm err}$ | $a_{3c,\rm err}$ | $a_{1s,\rm err}$ | $a_{2s,\rm err}$ | $a_{3s,\rm err}$ | | | |
| | [day] | BJD − 2455197.5 | [mag] | [mag] | [mag] | [mag] | [mag] | [mag] | [mag] | | | |
| 4043323684736161408 | 0.89117 | 2378.6109 | 17.6395 | -0.0179 | 0.0949 | -0.0118 | -0.0095 | 0.0000 | 0.0095 | 38 | 1.7 | 1.2 |
| | 0.00044 | 0.0033 | 0.0036 | 0.0047 | 0.0054 | 0.0048 | 0.0052 | 0.0045 | 0.0049 | | | |
| 4064671222613038720 | 0.69855 | 2232.4215 | 17.5815 | -0.0151 | 0.0949 | -0.0051 | 0.0107 | 0.0000 | 0.0027 | 30 | 1.7 | 1.2 |
| | 0.00032 | 0.0020 | 0.0023 | 0.0036 | 0.0037 | 0.0037 | 0.0031 | 0.0029 | 0.0030 | | | |
| 4117842745932000640 | 0.66775 | 2306.3396 | 18.3247 | 0.0242 | 0.0949 | 0.0091 | -0.0011 | 0.0000 | -0.0089 | 32 | 1.7 | 1.2 |
| | 0.00040 | 0.0022 | 0.0036 | 0.0059 | 0.0051 | 0.0041 | 0.0038 | 0.0043 | 0.0042 | | | |
| 2060076223135895936 | 0.366397 | 2230.65053 | 17.3734 | -0.0159 | 0.0949 | -0.0140 | 0.0019 | 0.0000 | 0.0057 | 42 | 1.7 | 1.2 |
| | 0.000071 | 0.00089 | 0.0029 | 0.0056 | 0.0056 | 0.0042 | 0.0032 | 0.0031 | 0.0037 | | | |
| 4118450363567306752 | 0.81241 | 2400.4801 | 17.6543 | 0.0169 | 0.0948 | 0.0053 | 0.0001 | 0.0000 | 0.0050 | 38 | 1.7 | 1.2 |
| | 0.00034 | 0.0024 | 0.0025 | 0.0038 | 0.0041 | 0.0035 | 0.0034 | 0.0032 | 0.0038 | | | |
| 4110445059963339264 | 0.97208 | 2286.6140 | 18.1807 | -0.0210 | 0.0947 | -0.0073 | 0.0067 | 0.0000 | -0.0028 | 31 | 1.7 | 1.2 |
| | 0.00070 | 0.0027 | 0.0024 | 0.0032 | 0.0033 | 0.0033 | 0.0036 | 0.0034 | 0.0033 | | | |
| 4119897664546481280 | 0.86212 | 2359.3597 | 17.5097 | 0.0263 | 0.0946 | 0.0172 | -0.0032 | 0.0000 | 0.0021 | 45 | 1.7 | 1.2 |
| | 0.00047 | 0.0017 | 0.0017 | 0.0024 | 0.0025 | 0.0021 | 0.0023 | 0.0021 | 0.0025 | | | |
| 5893822099469992320 | 0.79146 | 2134.1653 | 18.5093 | 0.0105 | 0.0946 | 0.0117 | -0.0090 | 0.0000 | 0.0117 | 46 | 1.7 | 1.2 |
| | 0.00037 | 0.0029 | 0.0037 | 0.0046 | 0.0053 | 0.0049 | 0.0057 | 0.0047 | 0.0048 | | | |
| 1809102278764951808 | 0.285391 | 2238.62702 | 17.6638 | -0.0031 | 0.0946 | -0.0071 | 0.0057 | 0.0000 | 0.0054 | 39 | 1.7 | 1.2 |
| | 0.000055 | 0.00070 | 0.0021 | 0.0028 | 0.0030 | 0.0030 | 0.0030 | 0.0027 | 0.0027 | | | |
| 259820095204356608 | 0.316389 | 2161.7573 | 18.1503 | -0.0046 | 0.0945 | -0.0028 | 0.0117 | 0.0000 | -0.0054 | 50 | 1.7 | 1.2 |
| | 0.000059 | 0.0010 | 0.0025 | 0.0040 | 0.0045 | 0.0034 | 0.0034 | 0.0030 | 0.0042 | | | |
| 445067811414955904 | 0.78164 | 2135.0702 | 18.6849 | 0.0055 | 0.0944 | 0.0034 | -0.0135 | 0.0000 | -0.0046 | 44 | 1.7 | 1.2 |
| | 0.00040 | 0.0023 | 0.0026 | 0.0038 | 0.0036 | 0.0034 | 0.0034 | 0.0034 | 0.0037 | | | |
| 4318036463047098240 | 0.314137 | 2119.4720 | 17.4927 | -0.0118 | 0.0944 | 0.0060 | -0.0126 | 0.0000 | -0.0045 | 37 | 1.7 | 1.1 |
| | 0.000058 | 0.0012 | 0.0033 | 0.0049 | 0.0066 | 0.0046 | 0.0051 | 0.0035 | 0.0054 | | | |
| 5938292323993830016 | 0.313719 | 2231.3130 | 18.2603 | 0.0204 | 0.0944 | 0.0063 | -0.0108 | 0.0000 | 0.0045 | 44 | 1.7 | 1.2 |
| | 0.000043 | 0.0012 | 0.0035 | 0.0052 | 0.0052 | 0.0046 | 0.0046 | 0.0045 | 0.0049 | | | |
| 4316136502611146624 | 0.89639 | 2066.2940 | 18.6573 | 0.0091 | 0.0943 | 0.0135 | 0.0019 | 0.0000 | -0.0076 | 43 | 1.7 | 1.2 |
| | 0.00054 | 0.0030 | 0.0030 | 0.0045 | 0.0038 | 0.0040 | 0.0037 | 0.0040 | 0.0036 | | | |
| 4175329057832249216 | 1.3760 | 2291.8575 | 18.3220 | -0.0018 | 0.0943 | -0.0242 | -0.0090 | 0.0000 | 0.0097 | 37 | 1.7 | 1.1 |
| | 0.0012 | 0.0077 | 0.0047 | 0.0083 | 0.0078 | 0.0063 | 0.0056 | 0.0053 | 0.0071 | | | |

Table S1: Continued.

| ***Gaia*** **DR3** | $P$ | $T_0$ | $\overline{G}$ | $a_{1c}$ | $a_{2c}$ | $a_{3c}$ | $a_{1s}$ | $a_{2s}$ | $a_{3s}$ | $N$ | $\hat{q}_{\rm min}$ | $\hat{q}_{\rm min}^{-1\sigma}$ |
|---|---|---|---|---|---|---|---|---|---|---|---|---|
| | $P_{\rm err}$ | $T_{0,\rm err}$ | $\overline{G}_{\rm err}$ | $a_{1c,\rm err}$ | $a_{2c,\rm err}$ | $a_{3c,\rm err}$ | $a_{1s,\rm err}$ | $a_{2s,\rm err}$ | $a_{3s,\rm err}$ | | | |
| | [day] | BJD − 2455197.5 | [mag] | [mag] | [mag] | [mag] | [mag] | [mag] | [mag] | | | |
| 5942571073496125568 | 0.47218 | 2164.5233 | 18.3159 | -0.0105 | 0.0942 | -0.0126 | -0.0010 | 0.0000 | -0.0031 | 51 | 1.7 | 1.2 |
| | 0.00013 | 0.0011 | 0.0023 | 0.0037 | 0.0031 | 0.0032 | 0.0026 | 0.0028 | 0.0026 | | | |
| 4321379974809694848 | 0.92030 | 2158.7781 | 17.0847 | 0.0159 | 0.0942 | -0.0035 | 0.0008 | 0.0000 | 0.0032 | 44 | 1.7 | 1.2 |
| | 0.00049 | 0.0019 | 0.0019 | 0.0026 | 0.0030 | 0.0025 | 0.0027 | 0.0023 | 0.0028 | | | |
| 2071059412252600576 | 0.49199 | 2215.9317 | 18.5184 | -0.0010 | 0.0942 | -0.0052 | 0.0139 | 0.0000 | -0.0070 | 43 | 1.7 | 1.2 |
| | 0.00021 | 0.0015 | 0.0025 | 0.0033 | 0.0038 | 0.0028 | 0.0037 | 0.0035 | 0.0046 | | | |
| 4096153603465854720 | 0.86104 | 2295.8124 | 18.2049 | 0.0240 | 0.0942 | 0.0060 | -0.0006 | 0.0000 | -0.0006 | 28 | 1.7 | 1.1 |
| | 0.00050 | 0.0025 | 0.0030 | 0.0049 | 0.0058 | 0.0045 | 0.0046 | 0.0034 | 0.0051 | | | |
| 1968171924489519488 | 0.271390 | 2234.08416 | 18.4071 | 0.0358 | 0.0942 | -0.0002 | 0.0057 | 0.0000 | -0.0037 | 50 | 1.7 | 1.2 |
| | 0.000047 | 0.00060 | 0.0019 | 0.0024 | 0.0026 | 0.0024 | 0.0028 | 0.0025 | 0.0028 | | | |
| 4123837592644301056 | 0.343691 | 2435.8365 | 18.7705 | 0.0174 | 0.0941 | -0.0033 | -0.0113 | 0.0000 | -0.0022 | 41 | 1.7 | 1.1 |
| | 0.000076 | 0.0011 | 0.0035 | 0.0044 | 0.0060 | 0.0053 | 0.0059 | 0.0039 | 0.0048 | | | |
| 4513206129189260032 | 0.64550 | 2124.7746 | 18.2330 | -0.0130 | 0.0941 | -0.0099 | -0.0013 | 0.0000 | -0.0024 | 44 | 1.7 | 1.2 |
| | 0.00027 | 0.0016 | 0.0023 | 0.0036 | 0.0033 | 0.0030 | 0.0026 | 0.0027 | 0.0030 | | | |
| 4068536693229974912 | 0.61348 | 2442.5391 | 18.5218 | -0.0152 | 0.0941 | -0.0062 | 0.0056 | 0.0000 | -0.0037 | 35 | 1.7 | 1.2 |
| | 0.00026 | 0.0021 | 0.0029 | 0.0037 | 0.0040 | 0.0039 | 0.0044 | 0.0040 | 0.0042 | | | |
| 4318085391317069568 | 0.42491 | 2138.3304 | 17.6525 | -0.0242 | 0.0939 | -0.0103 | -0.0050 | 0.0000 | -0.0032 | 41 | 1.7 | 1.2 |
| | 0.00013 | 0.0013 | 0.0029 | 0.0043 | 0.0039 | 0.0038 | 0.0036 | 0.0038 | 0.0037 | | | |
| 5836122100162716544 | 0.259831 | 2194.38785 | 18.3152 | -0.0049 | 0.0938 | -0.0050 | 0.0084 | 0.0000 | -0.0000 | 57 | 1.6 | 1.2 |
| | 0.000043 | 0.00054 | 0.0017 | 0.0025 | 0.0024 | 0.0023 | 0.0023 | 0.0024 | 0.0025 | | | |
| 4479262835157176448 | 0.313370 | 2282.98742 | 17.1939 | 0.0086 | 0.0938 | 0.0075 | 0.0022 | 0.0000 | 0.0030 | 46 | 1.6 | 1.2 |
| | 0.000058 | 0.00065 | 0.0018 | 0.0025 | 0.0034 | 0.0029 | 0.0031 | 0.0022 | 0.0028 | | | |
| 5935151607712641152 | 0.387107 | 2212.37008 | 17.6373 | 0.0154 | 0.0938 | -0.0030 | -0.0031 | 0.0000 | -0.0035 | 44 | 1.6 | 1.2 |
| | 0.000096 | 0.00063 | 0.0016 | 0.0024 | 0.0026 | 0.0028 | 0.0022 | 0.0019 | 0.0019 | | | |
| 5320709733731310720 | 0.272833 | 2187.16830 | 18.3314 | -0.0120 | 0.0938 | -0.0019 | 0.0148 | 0.0000 | -0.0040 | 37 | 1.6 | 1.2 |
| | 0.000059 | 0.00082 | 0.0025 | 0.0036 | 0.0036 | 0.0032 | 0.0034 | 0.0037 | 0.0038 | | | |
| 5826920940137873792 | 0.293029 | 2231.9881 | 18.8723 | -0.0213 | 0.0938 | -0.0088 | 0.0019 | 0.0000 | -0.0009 | 49 | 1.6 | 1.1 |
| | 0.000060 | 0.0010 | 0.0031 | 0.0044 | 0.0045 | 0.0041 | 0.0043 | 0.0041 | 0.0046 | | | |
| 4123238874157017984 | 0.346428 | 2429.8785 | 19.0220 | -0.0093 | 0.0938 | 0.0046 | 0.0168 | 0.0000 | -0.0100 | 40 | 1.6 | 1.1 |
| | 0.000083 | 0.0013 | 0.0036 | 0.0049 | 0.0058 | 0.0057 | 0.0056 | 0.0045 | 0.0049 | | | |

Table S1: Continued.

| ***Gaia*** **DR3** | $P$ | $T_0$ | $\overline{G}$ | $a_{1c}$ | $a_{2c}$ | $a_{3c}$ | $a_{1s}$ | $a_{2s}$ | $a_{3s}$ | $N$ | $\hat{q}_{\min}$ | $\hat{q}_{\min}^{-1\sigma}$ |
|---|---|---|---|---|---|---|---|---|---|---|---|---|
| | $P_{\rm err}$ | $T_{0,\rm err}$ | $\overline{G}_{\rm err}$ | $a_{1c,\rm err}$ | $a_{2c,\rm err}$ | $a_{3c,\rm err}$ | $a_{1s,\rm err}$ | $a_{2s,\rm err}$ | $a_{3s,\rm err}$ | | | |
| | [day] | BJD − 2455197.5 | [mag] | [mag] | [mag] | [mag] | [mag] | [mag] | [mag] | | | |
| 4064707987597656576 | 0.71082 | 2253.5672 | 17.7309 | 0.0217 | 0.0937 | 0.0033 | 0.0185 | 0.0000 | 0.0211 | 27 | 1.6 | 1.2 |
| | 0.00044 | 0.0043 | 0.0043 | 0.0068 | 0.0042 | 0.0039 | 0.0050 | 0.0080 | 0.0068 | | | |
| 5971314339012488832 | 0.40914 | 2286.6709 | 18.5141 | 0.0025 | 0.0937 | -0.0109 | 0.0036 | 0.0000 | -0.0019 | 35 | 1.6 | 1.2 |
| | 0.00013 | 0.0012 | 0.0025 | 0.0037 | 0.0034 | 0.0034 | 0.0031 | 0.0035 | 0.0035 | | | |
| 5867831598804630144 | 0.66770 | 2190.5757 | 18.6777 | 0.0141 | 0.0936 | 0.0102 | 0.0004 | 0.0000 | -0.0028 | 43 | 1.6 | 1.1 |
| | 0.00030 | 0.0025 | 0.0031 | 0.0045 | 0.0045 | 0.0041 | 0.0043 | 0.0042 | 0.0044 | | | |
| 4116793738878178304 | 0.63592 | 2453.6713 | 18.0681 | -0.0100 | 0.0936 | -0.0049 | 0.0014 | 0.0000 | 0.0012 | 56 | 1.6 | 1.2 |
| | 0.00023 | 0.0015 | 0.0019 | 0.0029 | 0.0028 | 0.0027 | 0.0026 | 0.0028 | 0.0029 | | | |
| 1825488163123795328 | 0.337134 | 2193.8147 | 18.8592 | -0.0145 | 0.0936 | -0.0152 | 0.0020 | 0.0000 | 0.0038 | 48 | 1.6 | 1.1 |
| | 0.000076 | 0.0011 | 0.0030 | 0.0050 | 0.0059 | 0.0051 | 0.0046 | 0.0035 | 0.0045 | | | |
| 4043982227758966528 | 1.10801 | 2352.9371 | 18.2308 | 0.0033 | 0.0935 | 0.0139 | -0.0029 | 0.0000 | 0.0099 | 39 | 1.6 | 1.1 |
| | 0.00066 | 0.0050 | 0.0037 | 0.0057 | 0.0055 | 0.0050 | 0.0046 | 0.0050 | 0.0057 | | | |
| 4363575893862498304 | 0.303803 | 2328.88963 | 17.3953 | -0.0181 | 0.0935 | -0.0012 | -0.0013 | 0.0000 | 0.0054 | 45 | 1.6 | 1.2 |
| | 0.000056 | 0.00069 | 0.0019 | 0.0027 | 0.0030 | 0.0026 | 0.0026 | 0.0025 | 0.0029 | | | |
| 6026017752571334400 | 0.320724 | 2300.6648 | 18.6999 | -0.0237 | 0.0935 | 0.0001 | 0.0051 | 0.0000 | -0.0081 | 42 | 1.6 | 1.1 |
| | 0.000085 | 0.0012 | 0.0035 | 0.0048 | 0.0058 | 0.0056 | 0.0054 | 0.0045 | 0.0051 | | | |
| 4151366060896624256 | 0.69710 | 2241.3239 | 17.7912 | -0.0024 | 0.0935 | 0.0008 | -0.0033 | 0.0000 | -0.0084 | 28 | 1.6 | 1.2 |
| | 0.00037 | 0.0019 | 0.0024 | 0.0039 | 0.0029 | 0.0026 | 0.0028 | 0.0034 | 0.0028 | | | |
| 4310698008860121216 | 0.75138 | 2242.7163 | 16.9948 | -0.0274 | 0.0935 | -0.0103 | 0.0068 | 0.0000 | -0.0001 | 31 | 1.6 | 1.2 |
| | 0.00044 | 0.0016 | 0.0021 | 0.0034 | 0.0034 | 0.0026 | 0.0025 | 0.0025 | 0.0026 | | | |
| 4120578330962979456 | 0.47945 | 2465.9817 | 17.9132 | 0.0270 | 0.0934 | 0.0086 | -0.0036 | 0.0000 | -0.0012 | 54 | 1.6 | 1.2 |
| | 0.00016 | 0.0011 | 0.0019 | 0.0029 | 0.0024 | 0.0026 | 0.0026 | 0.0028 | 0.0027 | | | |
| 5943198864598128000 | 0.391194 | 2272.87717 | 17.6130 | -0.0087 | 0.0933 | -0.0077 | -0.0006 | 0.0000 | -0.0009 | 39 | 1.6 | 1.2 |
| | 0.000094 | 0.00079 | 0.0016 | 0.0022 | 0.0027 | 0.0026 | 0.0024 | 0.0021 | 0.0024 | | | |
| 2057341939546521472 | 0.76659 | 2228.2136 | 18.2265 | -0.0078 | 0.0933 | 0.0040 | 0.0073 | 0.0000 | -0.0123 | 50 | 1.6 | 1.2 |
| | 0.00042 | 0.0016 | 0.0020 | 0.0025 | 0.0030 | 0.0024 | 0.0032 | 0.0026 | 0.0033 | | | |
| 5994289008090288640 | 0.347696 | 2044.6598 | 18.2809 | 0.0198 | 0.0932 | 0.0071 | 0.0123 | 0.0000 | -0.0002 | 49 | 1.6 | 1.1 |
| | 0.000070 | 0.0017 | 0.0044 | 0.0060 | 0.0066 | 0.0059 | 0.0064 | 0.0059 | 0.0066 | | | |
| 5881565705973807744 | 1.4167 | 2149.0462 | 17.3205 | 0.0035 | 0.0932 | 0.0083 | -0.0032 | 0.0000 | 0.0023 | 43 | 1.6 | 1.2 |
| | 0.0014 | 0.0034 | 0.0022 | 0.0033 | 0.0029 | 0.0027 | 0.0025 | 0.0027 | 0.0029 | | | |

Table S1: Continued.

| ***Gaia*** **DR3** | $P$<br>$P_{\rm err}$<br>[day] | $T_0$<br>$T_{0,\rm err}$<br>BJD − 2455197.5 | $\overline{G}$<br>$\overline{G}_{\rm err}$<br>[mag] | $a_{1\rm c}$<br>$a_{1\rm c,err}$<br>[mag] | $a_{2\rm c}$<br>$a_{2\rm c,err}$<br>[mag] | $a_{3\rm c}$<br>$a_{3\rm c,err}$<br>[mag] | $a_{1\rm s}$<br>$a_{1\rm s,err}$<br>[mag] | $a_{2\rm s}$<br>$a_{2\rm s,err}$<br>[mag] | $a_{3\rm s}$<br>$a_{3\rm s,err}$<br>[mag] | $N$ | $\hat{q}_{\rm min}$ | $\hat{q}_{\rm min}^{-1\sigma}$ |
|---|---|---|---|---|---|---|---|---|---|---|---|---|
| 2059063774754650880 | 0.91320 | 2218.5903 | 19.0771 | 0.0195 | 0.0932 | 0.0190 | 0.0015 | 0.0000 | -0.0075 | 52 | 1.6 | 1.1 |
| | 0.00051 | 0.0038 | 0.0038 | 0.0047 | 0.0057 | 0.0049 | 0.0060 | 0.0049 | 0.0050 | | | |
| 2168646566775705088 | 1.10239 | 2213.8016 | 17.3466 | -0.0117 | 0.0931 | -0.0013 | 0.0048 | 0.0000 | 0.0011 | 41 | 1.6 | 1.1 |
| | 0.00077 | 0.0026 | 0.0021 | 0.0025 | 0.0031 | 0.0029 | 0.0034 | 0.0026 | 0.0028 | | | |
| 5899729152678191488 | 0.380766 | 2127.7119 | 18.4759 | -0.0232 | 0.0931 | 0.0071 | 0.0107 | 0.0000 | -0.0033 | 47 | 1.6 | 1.1 |
| | 0.000096 | 0.0015 | 0.0031 | 0.0040 | 0.0049 | 0.0043 | 0.0050 | 0.0043 | 0.0045 | | | |
| 4067298574383612672 | 0.59294 | 2383.6211 | 17.8665 | 0.0201 | 0.0931 | 0.0134 | -0.0061 | 0.0000 | -0.0100 | 43 | 1.6 | 1.1 |
| | 0.00025 | 0.0017 | 0.0025 | 0.0040 | 0.0035 | 0.0032 | 0.0029 | 0.0032 | 0.0036 | | | |
| 5875031617582762624 | 0.55264 | 2199.8224 | 18.1768 | -0.0097 | 0.0930 | 0.0039 | 0.0107 | 0.0000 | 0.0056 | 45 | 1.6 | 1.1 |
| | 0.00024 | 0.0019 | 0.0030 | 0.0041 | 0.0035 | 0.0036 | 0.0044 | 0.0044 | 0.0043 | | | |
| 5992628371912715392 | 1.01903 | 2092.5844 | 17.7464 | -0.0103 | 0.0930 | 0.0027 | 0.0024 | 0.0000 | 0.0023 | 66 | 1.6 | 1.2 |
| | 0.00047 | 0.0017 | 0.0014 | 0.0022 | 0.0021 | 0.0020 | 0.0018 | 0.0018 | 0.0019 | | | |
| 4110726019578773120 | 0.61842 | 2314.7957 | 17.3155 | -0.0046 | 0.0930 | -0.0068 | 0.0000 | 0.0000 | -0.0028 | 49 | 1.6 | 1.2 |
| | 0.00027 | 0.0011 | 0.0015 | 0.0023 | 0.0023 | 0.0021 | 0.0019 | 0.0019 | 0.0021 | | | |
| 4293810854615414784 | 0.68068 | 2196.0645 | 16.6854 | -0.0035 | 0.0930 | 0.0102 | 0.0026 | 0.0000 | -0.0036 | 30 | 1.6 | 1.1 |
| | 0.00034 | 0.0019 | 0.0024 | 0.0033 | 0.0034 | 0.0029 | 0.0035 | 0.0034 | 0.0038 | | | |
| 6008216968556546432 | 0.311063 | 2079.19181 | 17.9034 | 0.0099 | 0.0930 | -0.0090 | -0.0163 | 0.0000 | 0.0085 | 41 | 1.6 | 1.1 |
| | 0.000078 | 0.00093 | 0.0029 | 0.0051 | 0.0053 | 0.0048 | 0.0036 | 0.0033 | 0.0036 | | | |
| 2033474222172499968 | 0.99435 | 2211.1893 | 17.7999 | 0.0143 | 0.0930 | 0.0044 | 0.0130 | 0.0000 | -0.0021 | 48 | 1.6 | 1.1 |
| | 0.00070 | 0.0031 | 0.0024 | 0.0036 | 0.0037 | 0.0033 | 0.0032 | 0.0033 | 0.0037 | | | |
| 4118634222571006976 | 0.48169 | 2388.0678 | 18.7444 | -0.0231 | 0.0930 | -0.0116 | 0.0057 | 0.0000 | -0.0009 | 43 | 1.6 | 1.0 |
| | 0.00015 | 0.0027 | 0.0050 | 0.0063 | 0.0075 | 0.0060 | 0.0081 | 0.0062 | 0.0079 | | | |
| 5937544248141179008 | 0.49960 | 2101.9102 | 16.9530 | 0.0150 | 0.0929 | -0.0030 | 0.0031 | 0.0000 | -0.0024 | 61 | 1.6 | 1.1 |
| | 0.00017 | 0.0012 | 0.0021 | 0.0039 | 0.0031 | 0.0024 | 0.0020 | 0.0024 | 0.0027 | | | |
| 5971704833097543168 | 0.83264 | 2274.0516 | 18.3054 | 0.0075 | 0.0929 | 0.0118 | -0.0091 | 0.0000 | 0.0051 | 41 | 1.6 | 1.1 |
| | 0.00059 | 0.0026 | 0.0027 | 0.0034 | 0.0039 | 0.0038 | 0.0042 | 0.0036 | 0.0035 | | | |
| 5972822177425474176 | 0.257090 | 2290.11042 | 16.9135 | -0.0089 | 0.0929 | -0.0018 | -0.0042 | 0.0000 | -0.0024 | 27 | 1.6 | 1.1 |
| | 0.000052 | 0.00049 | 0.0017 | 0.0027 | 0.0028 | 0.0022 | 0.0021 | 0.0022 | 0.0029 | | | |
| 5882261456319117440 | 0.339646 | 2122.7734 | 19.2242 | -0.0162 | 0.0929 | 0.0021 | 0.0108 | 0.0000 | 0.0055 | 46 | 1.6 | 1.1 |
| | 0.000094 | 0.0016 | 0.0042 | 0.0065 | 0.0057 | 0.0057 | 0.0052 | 0.0058 | 0.0055 | | | |

Table S1: Continued.

| ***Gaia*** **DR3** | $P$ | $T_0$ | $\overline{G}$ | $a_{1c}$ | $a_{2c}$ | $a_{3c}$ | $a_{1s}$ | $a_{2s}$ | $a_{3s}$ | $N$ | $\hat{q}_{\rm min}$ | $\hat{q}_{\rm min}^{-1\sigma}$ |
|---|---|---|---|---|---|---|---|---|---|---|---|---|
| | $P_{\rm err}$ | $T_{0,\rm err}$ | $\overline{G}_{\rm err}$ | $a_{1c,\rm err}$ | $a_{2c,\rm err}$ | $a_{3c,\rm err}$ | $a_{1s,\rm err}$ | $a_{2s,\rm err}$ | $a_{3s,\rm err}$ | | | |
| | [day] | BJD – 2455197.5 | [mag] | [mag] | [mag] | [mag] | [mag] | [mag] | [mag] | | | |
| 4163226698979126784 | 0.362717 | 2386.19380 | 18.5932 | -0.0115 | 0.0928 | -0.0024 | 0.0113 | 0.0000 | 0.0003 | 51 | 1.6 | 1.1 |
| | 0.000087 | 0.00075 | 0.0017 | 0.0026 | 0.0025 | 0.0024 | 0.0022 | 0.0023 | 0.0024 | | | |
| 4056840530856775168 | 0.74118 | 2389.9054 | 17.6444 | -0.0102 | 0.0928 | 0.0055 | -0.0056 | 0.0000 | 0.0034 | 43 | 1.6 | 1.1 |
| | 0.00026 | 0.0020 | 0.0025 | 0.0034 | 0.0032 | 0.0028 | 0.0030 | 0.0031 | 0.0037 | | | |
| 3020455473403312128 | 0.343936 | 2306.98800 | 17.6805 | -0.0219 | 0.0928 | 0.0024 | 0.0083 | 0.0000 | -0.0006 | 33 | 1.6 | 1.1 |
| | 0.000091 | 0.00087 | 0.0024 | 0.0038 | 0.0037 | 0.0033 | 0.0030 | 0.0029 | 0.0033 | | | |
| 4121045309772537600 | 0.72209 | 2304.7961 | 18.2669 | 0.0150 | 0.0927 | -0.0007 | -0.0040 | 0.0000 | -0.0087 | 39 | 1.6 | 1.1 |
| | 0.00040 | 0.0022 | 0.0024 | 0.0034 | 0.0035 | 0.0032 | 0.0033 | 0.0034 | 0.0036 | | | |
| 4515710546088089344 | 1.3963 | 2200.8673 | 18.1871 | 0.0279 | 0.0926 | -0.0046 | 0.0054 | 0.0000 | 0.0020 | 53 | 1.6 | 1.1 |
| | 0.0013 | 0.0050 | 0.0029 | 0.0039 | 0.0039 | 0.0043 | 0.0042 | 0.0042 | 0.0038 | | | |
| 5328547537954751232 | 1.04209 | 2266.4639 | 17.6644 | 0.0113 | 0.0926 | 0.0050 | 0.0072 | 0.0000 | 0.0088 | 40 | 1.6 | 1.1 |
| | 0.00068 | 0.0033 | 0.0025 | 0.0029 | 0.0042 | 0.0039 | 0.0041 | 0.0034 | 0.0040 | | | |
| 1826661857416121344 | 0.275488 | 2127.9002 | 18.2022 | -0.0178 | 0.0926 | 0.0069 | 0.0050 | 0.0000 | -0.0049 | 54 | 1.6 | 1.1 |
| | 0.000052 | 0.0011 | 0.0034 | 0.0049 | 0.0049 | 0.0045 | 0.0046 | 0.0048 | 0.0052 | | | |
| 5886930871683919232 | 0.58123 | 2182.6683 | 18.6587 | 0.0134 | 0.0925 | 0.0023 | 0.0035 | 0.0000 | 0.0084 | 45 | 1.6 | 1.1 |
| | 0.00021 | 0.0016 | 0.0026 | 0.0045 | 0.0035 | 0.0035 | 0.0027 | 0.0032 | 0.0032 | | | |
| 4044188931802966400 | 1.05793 | 2427.6840 | 17.9532 | 0.0263 | 0.0925 | 0.0085 | -0.0209 | 0.0000 | -0.0016 | 56 | 1.6 | 1.1 |
| | 0.00065 | 0.0025 | 0.0020 | 0.0028 | 0.0027 | 0.0033 | 0.0028 | 0.0029 | 0.0025 | | | |
| 4117616040406930688 | 0.67017 | 2411.4473 | 18.2388 | 0.0075 | 0.0925 | 0.0025 | 0.0039 | 0.0000 | -0.0011 | 47 | 1.6 | 1.1 |
| | 0.00026 | 0.0015 | 0.0020 | 0.0028 | 0.0029 | 0.0028 | 0.0029 | 0.0027 | 0.0029 | | | |
| 5880978326225888000 | 0.99953 | 2104.2498 | 19.4702 | 0.0174 | 0.0925 | 0.0046 | -0.0009 | 0.0000 | -0.0040 | 38 | 1.6 | 1.1 |
| | 0.00064 | 0.0026 | 0.0022 | 0.0032 | 0.0041 | 0.0037 | 0.0037 | 0.0027 | 0.0035 | | | |
| 4118098966636199040 | 0.60001 | 2416.1903 | 17.9209 | 0.0048 | 0.0925 | -0.0092 | 0.0027 | 0.0000 | 0.0064 | 49 | 1.6 | 1.1 |
| | 0.00020 | 0.0013 | 0.0020 | 0.0028 | 0.0031 | 0.0027 | 0.0028 | 0.0025 | 0.0028 | | | |
| 204842903200280064 | 0.37514 | 2256.4455 | 18.5973 | 0.0301 | 0.0925 | -0.0057 | -0.0052 | 0.0000 | -0.0048 | 46 | 1.6 | 1.1 |
| | 0.00012 | 0.0016 | 0.0036 | 0.0053 | 0.0056 | 0.0063 | 0.0051 | 0.0048 | 0.0045 | | | |
| 5981814464556498304 | 0.84923 | 2160.5058 | 18.0740 | 0.0121 | 0.0925 | 0.0014 | -0.0023 | 0.0000 | -0.0019 | 54 | 1.6 | 1.1 |
| | 0.00045 | 0.0025 | 0.0025 | 0.0039 | 0.0038 | 0.0037 | 0.0032 | 0.0031 | 0.0033 | | | |
| 5972087703660023168 | 0.327445 | 2286.11996 | 18.2167 | -0.0084 | 0.0925 | 0.0004 | -0.0063 | 0.0000 | 0.0036 | 55 | 1.6 | 1.1 |
| | 0.000084 | 0.00090 | 0.0022 | 0.0028 | 0.0038 | 0.0033 | 0.0036 | 0.0026 | 0.0032 | | | |

Table S1: Continued.

| ***Gaia*** DR3 | $P$<br>$P_{\rm err}$<br>[day] | $T_0$<br>$T_{0,\rm err}$<br>BJD − 2455197.5 | $\overline{G}$<br>$\overline{G}_{\rm err}$<br>[mag] | $a_{1\rm c}$<br>$a_{1\rm c,err}$<br>[mag] | $a_{2\rm c}$<br>$a_{2\rm c,err}$<br>[mag] | $a_{3\rm c}$<br>$a_{3\rm c,err}$<br>[mag] | $a_{1\rm s}$<br>$a_{1\rm s,err}$<br>[mag] | $a_{2\rm s}$<br>$a_{2\rm s,err}$<br>[mag] | $a_{3\rm s}$<br>$a_{3\rm s,err}$<br>[mag] | $N$ | $\hat{q}_{\rm min}$ | $\hat{q}_{\rm min}^{-1\sigma}$ |
|---|---|---|---|---|---|---|---|---|---|---|---|---|
| 5827299275184119680 | 0.318691 | 2170.42691 | 18.1563 | -0.0267 | 0.0924 | 0.0036 | -0.0024 | 0.0000 | -0.0010 | 41 | 1.6 | 1.1 |
| | 0.000086 | 0.00089 | 0.0023 | 0.0033 | 0.0034 | 0.0029 | 0.0033 | 0.0033 | 0.0036 | | | |
| 248990352345204736 | 0.283507 | 2118.51277 | 18.5419 | 0.0114 | 0.0924 | 0.0111 | 0.0160 | 0.0000 | -0.0150 | 35 | 1.5 | 1.1 |
| | 0.000070 | 0.00071 | 0.0026 | 0.0029 | 0.0040 | 0.0030 | 0.0046 | 0.0029 | 0.0041 | | | |
| 447431550955645056 | 0.55883 | 2162.64809 | 17.0402 | 0.0127 | 0.0924 | -0.0002 | -0.0014 | 0.0000 | -0.0068 | 43 | 1.5 | 1.1 |
| | 0.00023 | 0.00099 | 0.0015 | 0.0020 | 0.0019 | 0.0021 | 0.0019 | 0.0021 | 0.0020 | | | |
| 4320874749205944064 | 1.1894 | 2152.7639 | 18.0463 | -0.0169 | 0.0923 | -0.0133 | 0.0118 | 0.0000 | 0.0031 | 36 | 1.5 | 1.1 |
| | 0.0010 | 0.0051 | 0.0037 | 0.0038 | 0.0052 | 0.0044 | 0.0062 | 0.0042 | 0.0041 | | | |
| 4143871141177911424 | 0.50948 | 2285.8313 | 18.9006 | 0.0179 | 0.0922 | 0.0117 | 0.0114 | 0.0000 | 0.0108 | 29 | 1.5 | 1.1 |
| | 0.00024 | 0.0023 | 0.0036 | 0.0057 | 0.0057 | 0.0049 | 0.0043 | 0.0048 | 0.0054 | | | |
| 5941303409633668352 | 0.328864 | 2098.37619 | 17.8166 | -0.0137 | 0.0922 | 0.0014 | 0.0165 | 0.0000 | -0.0037 | 66 | 1.5 | 1.1 |
| | 0.000045 | 0.00073 | 0.0021 | 0.0034 | 0.0041 | 0.0033 | 0.0031 | 0.0024 | 0.0033 | | | |
| 2057701342412484864 | 0.43729 | 2226.6597 | 18.9683 | -0.0116 | 0.0922 | -0.0083 | 0.0058 | 0.0000 | 0.0064 | 44 | 1.5 | 1.1 |
| | 0.00013 | 0.0015 | 0.0029 | 0.0041 | 0.0041 | 0.0039 | 0.0040 | 0.0040 | 0.0040 | | | |
| 4093878473392045184 | 1.1766 | 2277.7125 | 17.1437 | 0.0176 | 0.0922 | 0.0038 | 0.0019 | 0.0000 | 0.0057 | 29 | 1.5 | 1.1 |
| | 0.0015 | 0.0028 | 0.0022 | 0.0036 | 0.0031 | 0.0031 | 0.0025 | 0.0027 | 0.0027 | | | |
| 2070452584917307392 | 0.78219 | 2233.6351 | 18.9005 | -0.0117 | 0.0922 | -0.0058 | -0.0037 | 0.0000 | -0.0014 | 37 | 1.5 | 1.1 |
| | 0.00054 | 0.0025 | 0.0029 | 0.0035 | 0.0042 | 0.0040 | 0.0045 | 0.0036 | 0.0038 | | | |
| 4119483904538549888 | 0.70011 | 2279.5847 | 18.9214 | -0.0107 | 0.0922 | -0.0056 | -0.0078 | 0.0000 | -0.0010 | 34 | 1.5 | 1.1 |
| | 0.00037 | 0.0020 | 0.0024 | 0.0038 | 0.0034 | 0.0032 | 0.0030 | 0.0032 | 0.0029 | | | |
| 4117177747570283648 | 0.68644 | 2397.0437 | 18.2191 | 0.0265 | 0.0922 | 0.0003 | 0.0039 | 0.0000 | -0.0029 | 47 | 1.5 | 1.1 |
| | 0.00028 | 0.0021 | 0.0023 | 0.0034 | 0.0031 | 0.0031 | 0.0032 | 0.0036 | 0.0035 | | | |
| 2082840168254168704 | 0.309990 | 2235.16632 | 18.2965 | 0.0182 | 0.0921 | -0.0053 | -0.0053 | 0.0000 | -0.0024 | 42 | 1.5 | 1.1 |
| | 0.000057 | 0.00098 | 0.0026 | 0.0036 | 0.0036 | 0.0033 | 0.0036 | 0.0037 | 0.0039 | | | |
| 2166489187524929152 | 0.66296 | 2263.3103 | 18.7785 | -0.0102 | 0.0921 | 0.0104 | -0.0112 | 0.0000 | 0.0088 | 45 | 1.5 | 1.1 |
| | 0.00034 | 0.0023 | 0.0029 | 0.0042 | 0.0038 | 0.0040 | 0.0037 | 0.0041 | 0.0034 | | | |
| 5834715545522454016 | 0.341319 | 2165.5997 | 18.1042 | 0.0023 | 0.0919 | 0.0120 | 0.0120 | 0.0000 | -0.0061 | 57 | 1.5 | 1.1 |
| | 0.000065 | 0.0012 | 0.0029 | 0.0042 | 0.0043 | 0.0042 | 0.0039 | 0.0041 | 0.0042 | | | |
| 2030386553000124928 | 0.76120 | 2234.9132 | 18.7322 | -0.0095 | 0.0919 | -0.0076 | 0.0161 | 0.0000 | -0.0021 | 50 | 1.5 | 1.1 |
| | 0.00040 | 0.0022 | 0.0024 | 0.0036 | 0.0035 | 0.0036 | 0.0032 | 0.0034 | 0.0033 | | | |

Table S1: Continued.

| ***Gaia*** **DR3** | $P$<br>$P_{\rm err}$<br>[day] | $T_0$<br>$T_{0,\rm err}$<br>BJD − 2455197.5 | $\overline{G}$<br>$\overline{G}_{\rm err}$<br>[mag] | $a_{1\rm c}$<br>$a_{1\rm c,err}$<br>[mag] | $a_{2\rm c}$<br>$a_{2\rm c,err}$<br>[mag] | $a_{3\rm c}$<br>$a_{3\rm c,err}$<br>[mag] | $a_{1\rm s}$<br>$a_{1\rm s,err}$<br>[mag] | $a_{2\rm s}$<br>$a_{2\rm s,err}$<br>[mag] | $a_{3\rm s}$<br>$a_{3\rm s,err}$<br>[mag] | $N$ | $\hat{q}_{\rm min}$ | $\hat{q}_{\rm min}^{-1\sigma}$ |
|---|---|---|---|---|---|---|---|---|---|---|---|---|
| 5625094134724407296 | 0.56758 | 2224.3793 | 18.3033 | 0.0102 | 0.0919 | -0.0001 | -0.0043 | 0.0000 | 0.0121 | 46 | 1.5 | 1.1 |
| | 0.00016 | 0.0014 | 0.0022 | 0.0031 | 0.0031 | 0.0030 | 0.0030 | 0.0029 | 0.0029 | | | |
| 5980528413934936960 | 0.98810 | 2334.1628 | 18.4741 | 0.0024 | 0.0918 | 0.0073 | 0.0055 | 0.0000 | -0.0057 | 49 | 1.5 | 1.1 |
| | 0.00071 | 0.0025 | 0.0020 | 0.0031 | 0.0032 | 0.0031 | 0.0028 | 0.0029 | 0.0031 | | | |
| 207660947209655552 | 0.34303 | 2256.0130 | 17.9652 | -0.0316 | 0.0918 | -0.0060 | -0.0181 | 0.0000 | -0.0012 | 37 | 1.5 | 1.1 |
| | 0.00011 | 0.0013 | 0.0032 | 0.0058 | 0.0049 | 0.0044 | 0.0034 | 0.0036 | 0.0038 | | | |
| 4143833001843654912 | 0.90265 | 2275.5808 | 16.6804 | 0.0087 | 0.0917 | 0.0027 | 0.0031 | 0.0000 | 0.0012 | 30 | 1.5 | 1.1 |
| | 0.00050 | 0.0020 | 0.0018 | 0.0023 | 0.0028 | 0.0023 | 0.0027 | 0.0023 | 0.0027 | | | |
| 5976765133512018048 | 0.77977 | 2249.6368 | 19.2559 | -0.0182 | 0.0917 | -0.0050 | -0.0063 | 0.0000 | -0.0042 | 42 | 1.5 | 1.0 |
| | 0.00058 | 0.0046 | 0.0047 | 0.0059 | 0.0067 | 0.0069 | 0.0071 | 0.0065 | 0.0059 | | | |
| 1825852380648525568 | 0.78382 | 2142.4854 | 19.3507 | 0.0038 | 0.0917 | -0.0151 | -0.0085 | 0.0000 | 0.0110 | 43 | 1.5 | 1.1 |
| | 0.00047 | 0.0030 | 0.0032 | 0.0045 | 0.0047 | 0.0044 | 0.0046 | 0.0044 | 0.0042 | | | |
| 5874498384473949952 | 0.327224 | 2229.03668 | 17.4565 | 0.0139 | 0.0917 | 0.0006 | -0.0179 | 0.0000 | -0.0003 | 57 | 1.5 | 1.1 |
| | 0.000058 | 0.00092 | 0.0023 | 0.0035 | 0.0037 | 0.0033 | 0.0031 | 0.0028 | 0.0034 | | | |
| 4119844368194081536 | 0.89974 | 2443.3744 | 18.2460 | 0.0120 | 0.0917 | -0.0032 | 0.0006 | 0.0000 | 0.0008 | 56 | 1.5 | 1.1 |
| | 0.00048 | 0.0022 | 0.0020 | 0.0030 | 0.0032 | 0.0028 | 0.0028 | 0.0026 | 0.0031 | | | |
| 4049886948789883520 | 0.89627 | 2247.2411 | 16.8148 | 0.0047 | 0.0917 | 0.0037 | -0.0024 | 0.0000 | -0.0080 | 27 | 1.5 | 1.1 |
| | 0.00058 | 0.0020 | 0.0019 | 0.0023 | 0.0029 | 0.0027 | 0.0029 | 0.0023 | 0.0027 | | | |
| 5320873629683093632 | 0.315678 | 2220.1434 | 17.7923 | -0.0107 | 0.0916 | -0.0047 | 0.0005 | 0.0000 | 0.0105 | 37 | 1.5 | 1.1 |
| | 0.000085 | 0.0011 | 0.0027 | 0.0037 | 0.0036 | 0.0038 | 0.0038 | 0.0039 | 0.0037 | | | |
| 4117606965114089600 | 0.74470 | 2481.2715 | 17.7954 | -0.0059 | 0.0916 | -0.0091 | 0.0016 | 0.0000 | -0.0008 | 57 | 1.5 | 1.1 |
| | 0.00029 | 0.0014 | 0.0015 | 0.0020 | 0.0023 | 0.0021 | 0.0023 | 0.0021 | 0.0023 | | | |
| 2167505033188323968 | 1.06422 | 2213.7029 | 18.3751 | 0.0271 | 0.0916 | 0.0196 | 0.0041 | 0.0000 | -0.0068 | 38 | 1.5 | 1.0 |
| | 0.00094 | 0.0046 | 0.0043 | 0.0037 | 0.0058 | 0.0046 | 0.0080 | 0.0047 | 0.0053 | | | |
| 2064907060581325312 | 0.88490 | 2246.4906 | 18.5919 | 0.0151 | 0.0916 | 0.0125 | 0.0011 | 0.0000 | -0.0077 | 46 | 1.5 | 1.1 |
| | 0.00050 | 0.0030 | 0.0027 | 0.0037 | 0.0037 | 0.0039 | 0.0039 | 0.0039 | 0.0037 | | | |
| 5963284055800046208 | 0.64241 | 2260.0021 | 18.2018 | 0.0030 | 0.0916 | 0.0054 | -0.0120 | 0.0000 | 0.0002 | 43 | 1.5 | 1.1 |
| | 0.00044 | 0.0018 | 0.0026 | 0.0035 | 0.0041 | 0.0036 | 0.0038 | 0.0033 | 0.0037 | | | |
| 5961314860547542272 | 0.56659 | 2442.4475 | 18.3929 | 0.0214 | 0.0915 | 0.0115 | -0.0016 | 0.0000 | -0.0004 | 44 | 1.5 | 1.0 |
| | 0.00019 | 0.0027 | 0.0041 | 0.0068 | 0.0059 | 0.0058 | 0.0048 | 0.0052 | 0.0053 | | | |

Table S1: Continued.

| ***Gaia*** **DR3** | $P$ | $T_0$ | $\overline{G}$ | $a_{1c}$ | $a_{2c}$ | $a_{3c}$ | $a_{1s}$ | $a_{2s}$ | $a_{3s}$ | $N$ | $\hat{q}_{min}$ | $\hat{q}_{min}^{-1\sigma}$ |
|---|---|---|---|---|---|---|---|---|---|---|---|---|
| | $P_{err}$ | $T_{0,err}$ | $\overline{G}_{err}$ | $a_{1c,err}$ | $a_{2c,err}$ | $a_{3c,err}$ | $a_{1s,err}$ | $a_{2s,err}$ | $a_{3s,err}$ | | | |
| | [day] | BJD − 2455197.5 | [mag] | [mag] | [mag] | [mag] | [mag] | [mag] | [mag] | | | |
| 4041781997731010560 | 0.54160 | 2453.7587 | 17.8955 | -0.0382 | 0.0915 | -0.0216 | 0.0024 | 0.0000 | 0.0054 | 47 | 1.5 | 1.1 |
| | 0.00023 | 0.0018 | 0.0026 | 0.0035 | 0.0035 | 0.0035 | 0.0039 | 0.0038 | 0.0037 | | | |
| 5937640004367021056 | 0.65716 | 2267.8089 | 17.2796 | 0.0104 | 0.0915 | 0.0007 | 0.0041 | 0.0000 | 0.0014 | 41 | 1.5 | 1.1 |
| | 0.00034 | 0.0015 | 0.0020 | 0.0031 | 0.0029 | 0.0027 | 0.0026 | 0.0027 | 0.0027 | | | |
| 5941788874056868224 | 0.66697 | 2188.1619 | 18.0719 | -0.0183 | 0.0915 | -0.0004 | 0.0070 | 0.0000 | -0.0046 | 37 | 1.5 | 1.1 |
| | 0.00033 | 0.0017 | 0.0024 | 0.0032 | 0.0035 | 0.0032 | 0.0033 | 0.0029 | 0.0032 | | | |
| 5988085121143687936 | 0.76055 | 2088.7905 | 17.4711 | -0.0100 | 0.0915 | -0.0047 | -0.0056 | 0.0000 | -0.0044 | 45 | 1.5 | 1.1 |
| | 0.00042 | 0.0019 | 0.0021 | 0.0031 | 0.0029 | 0.0027 | 0.0027 | 0.0028 | 0.0030 | | | |
| 276523566614691328 | 0.351595 | 2162.45647 | 18.2221 | -0.0136 | 0.0914 | 0.0025 | 0.0095 | 0.0000 | -0.0066 | 74 | 1.5 | 1.1 |
| | 0.000065 | 0.00078 | 0.0019 | 0.0029 | 0.0034 | 0.0030 | 0.0029 | 0.0024 | 0.0028 | | | |
| 5996899798450078336 | 0.33411 | 2048.4372 | 18.3829 | 0.0092 | 0.0914 | -0.0079 | -0.0055 | 0.0000 | 0.0004 | 51 | 1.5 | 1.1 |
| | 0.00012 | 0.0010 | 0.0020 | 0.0029 | 0.0035 | 0.0034 | 0.0031 | 0.0033 | 0.0031 | | | |
| 2021284349073934464 | 0.360199 | 2247.96470 | 18.6175 | -0.0143 | 0.0914 | 0.0012 | -0.0039 | 0.0000 | 0.0029 | 86 | 1.5 | 1.1 |
| | 0.000074 | 0.00084 | 0.0019 | 0.0027 | 0.0026 | 0.0027 | 0.0026 | 0.0028 | 0.0026 | | | |
| 2068602141207393536 | 0.79395 | 2213.8988 | 17.8619 | -0.0036 | 0.0914 | -0.0047 | 0.0186 | 0.0000 | 0.0010 | 43 | 1.5 | 1.1 |
| | 0.00041 | 0.0023 | 0.0026 | 0.0038 | 0.0038 | 0.0036 | 0.0035 | 0.0034 | 0.0037 | | | |
| 4111120125751883136 | 1.03307 | 2336.5157 | 17.4954 | -0.0077 | 0.0913 | -0.0012 | 0.0004 | 0.0000 | 0.0050 | 59 | 1.5 | 1.1 |
| | 0.00079 | 0.0020 | 0.0015 | 0.0021 | 0.0025 | 0.0021 | 0.0022 | 0.0019 | 0.0022 | | | |
| 4099704411943299584 | 0.45503 | 2208.61771 | 18.2109 | -0.0055 | 0.0913 | -0.0086 | -0.0138 | 0.0000 | -0.0002 | 28 | 1.5 | 1.1 |
| | 0.00012 | 0.00098 | 0.0018 | 0.0027 | 0.0029 | 0.0027 | 0.0025 | 0.0024 | 0.0026 | | | |
| 2070671800043522816 | 0.72265 | 2211.5414 | 18.4693 | 0.0047 | 0.0913 | 0.0113 | -0.0185 | 0.0000 | -0.0002 | 48 | 1.5 | 1.1 |
| | 0.00041 | 0.0017 | 0.0019 | 0.0028 | 0.0027 | 0.0028 | 0.0027 | 0.0028 | 0.0028 | | | |
| 4302041656898064000 | 0.270171 | 2173.91683 | 18.2411 | -0.0086 | 0.0913 | -0.0029 | 0.0165 | 0.0000 | -0.0122 | 39 | 1.5 | 1.0 |
| | 0.000065 | 0.00097 | 0.0032 | 0.0041 | 0.0043 | 0.0039 | 0.0046 | 0.0043 | 0.0049 | | | |
| 247176849656507392 | 0.46842 | 2139.23604 | 17.4955 | 0.0104 | 0.0913 | -0.0033 | 0.0055 | 0.0000 | 0.0015 | 65 | 1.5 | 1.1 |
| | 0.00015 | 0.00083 | 0.0015 | 0.0021 | 0.0022 | 0.0022 | 0.0021 | 0.0020 | 0.0020 | | | |
| 4312619645957182592 | 0.61736 | 2228.1260 | 17.6956 | -0.0117 | 0.0912 | -0.0077 | -0.0032 | 0.0000 | -0.0012 | 27 | 1.5 | 1.1 |
| | 0.00035 | 0.0019 | 0.0023 | 0.0033 | 0.0027 | 0.0033 | 0.0036 | 0.0041 | 0.0038 | | | |
| 4044125336065254784 | 0.392346 | 2389.7711 | 17.7688 | 0.0015 | 0.0912 | -0.0035 | -0.0128 | 0.0000 | 0.0026 | 53 | 1.5 | 1.1 |
| | 0.000082 | 0.0010 | 0.0021 | 0.0035 | 0.0033 | 0.0029 | 0.0026 | 0.0026 | 0.0030 | | | |

Table S1: Continued.

| ***Gaia*** **DR3** | $P$ | $T_0$ | $\overline{G}$ | $a_{1c}$ | $a_{2c}$ | $a_{3c}$ | $a_{1s}$ | $a_{2s}$ | $a_{3s}$ | $N$ | $\hat{q}_{min}$ | $\hat{q}_{min}^{-1\sigma}$ |
|---|---|---|---|---|---|---|---|---|---|---|---|---|
| | $P_{err}$ | $T_{0,err}$ | $\overline{G}_{err}$ | $a_{1c,err}$ | $a_{2c,err}$ | $a_{3c,err}$ | $a_{1s,err}$ | $a_{2s,err}$ | $a_{3s,err}$ | | | |
| | [day] | BJD − 2455197.5 | [mag] | [mag] | [mag] | [mag] | [mag] | [mag] | [mag] | | | |
| 154974759483084800 | 0.328355 | 2227.04151 | 17.9959 | 0.0114 | 0.0911 | -0.0025 | -0.0037 | 0.0000 | 0.0004 | 43 | 1.5 | 1.1 |
| | 0.000089 | 0.00098 | 0.0024 | 0.0034 | 0.0036 | 0.0032 | 0.0034 | 0.0032 | 0.0036 | | | |
| 4057433962273137024 | 1.3856 | 2395.0994 | 17.4323 | -0.0302 | 0.0911 | -0.0113 | -0.0044 | 0.0000 | 0.0045 | 38 | 1.5 | 1.1 |
| | 0.0015 | 0.0036 | 0.0021 | 0.0027 | 0.0030 | 0.0026 | 0.0032 | 0.0028 | 0.0030 | | | |
| 5900910715358995712 | 0.330491 | 2073.81110 | 18.2893 | 0.0125 | 0.0911 | 0.0039 | 0.0034 | 0.0000 | -0.0059 | 47 | 1.5 | 1.1 |
| | 0.000083 | 0.00082 | 0.0021 | 0.0028 | 0.0036 | 0.0034 | 0.0035 | 0.0026 | 0.0029 | | | |
| 5971306058314604416 | 0.73353 | 2252.1664 | 18.0904 | -0.0072 | 0.0911 | -0.0091 | -0.0035 | 0.0000 | 0.0069 | 45 | 1.5 | 1.0 |
| | 0.00052 | 0.0025 | 0.0027 | 0.0039 | 0.0038 | 0.0035 | 0.0038 | 0.0038 | 0.0042 | | | |
| 5863313671165798400 | 0.42933 | 2250.1111 | 19.2756 | -0.0553 | 0.0910 | -0.0087 | 0.0037 | 0.0000 | 0.0024 | 51 | 1.5 | 1.1 |
| | 0.00012 | 0.0012 | 0.0024 | 0.0033 | 0.0035 | 0.0032 | 0.0033 | 0.0032 | 0.0034 | | | |
| 5938179658413745408 | 0.38333 | 2281.3821 | 18.1852 | -0.0140 | 0.0910 | -0.0054 | 0.0117 | 0.0000 | -0.0009 | 43 | 1.5 | 1.0 |
| | 0.00012 | 0.0012 | 0.0027 | 0.0042 | 0.0044 | 0.0037 | 0.0037 | 0.0034 | 0.0042 | | | |
| 251995150125170176 | 0.55580 | 2107.9947 | 19.2141 | 0.0221 | 0.0910 | 0.0086 | -0.0039 | 0.0000 | 0.0015 | 44 | 1.5 | 1.0 |
| | 0.00024 | 0.0018 | 0.0027 | 0.0042 | 0.0041 | 0.0041 | 0.0035 | 0.0036 | 0.0037 | | | |
| 5307187600455149440 | 0.48955 | 2088.1761 | 18.3497 | 0.0392 | 0.0910 | 0.0018 | -0.0218 | 0.0000 | 0.0032 | 51 | 1.5 | 1.1 |
| | 0.00013 | 0.0014 | 0.0022 | 0.0037 | 0.0035 | 0.0031 | 0.0026 | 0.0027 | 0.0029 | | | |
| 5972041597240517888 | 0.90025 | 2264.2455 | 17.8021 | -0.0090 | 0.0910 | -0.0036 | -0.0045 | 0.0000 | 0.0018 | 48 | 1.5 | 1.1 |
| | 0.00065 | 0.0021 | 0.0019 | 0.0025 | 0.0025 | 0.0023 | 0.0027 | 0.0026 | 0.0028 | | | |
| 5972962197660553344 | 0.62191 | 2300.5718 | 18.8714 | -0.0112 | 0.0909 | -0.0048 | 0.0161 | 0.0000 | -0.0063 | 69 | 1.5 | 1.0 |
| | 0.00029 | 0.0020 | 0.0025 | 0.0035 | 0.0035 | 0.0038 | 0.0035 | 0.0036 | 0.0033 | | | |
| 183793676507073536 | 0.80890 | 2255.7543 | 17.8467 | 0.0097 | 0.0909 | 0.0114 | -0.0004 | 0.0000 | 0.0020 | 29 | 1.5 | 1.1 |
| | 0.00055 | 0.0021 | 0.0024 | 0.0036 | 0.0032 | 0.0026 | 0.0029 | 0.0031 | 0.0033 | | | |
| 5834273546240620160 | 0.328038 | 2172.67542 | 17.0265 | -0.0015 | 0.0909 | -0.0020 | 0.0074 | 0.0000 | 0.0000 | 48 | 1.5 | 1.1 |
| | 0.000069 | 0.00073 | 0.0019 | 0.0030 | 0.0029 | 0.0025 | 0.0022 | 0.0023 | 0.0025 | | | |
| 2075326032771354752 | 0.267476 | 2184.59330 | 18.5656 | -0.0132 | 0.0908 | -0.0028 | -0.0138 | 0.0000 | 0.0002 | 48 | 1.4 | 1.0 |
| | 0.000054 | 0.00095 | 0.0030 | 0.0043 | 0.0043 | 0.0039 | 0.0041 | 0.0040 | 0.0044 | | | |
| 5330205116149118208 | 0.54348 | 2203.8449 | 19.1236 | -0.0083 | 0.0908 | 0.0067 | 0.0199 | 0.0000 | 0.0080 | 40 | 1.4 | 1.0 |
| | 0.00019 | 0.0022 | 0.0034 | 0.0050 | 0.0051 | 0.0049 | 0.0046 | 0.0046 | 0.0049 | | | |
| 5977757030454814848 | 0.359105 | 2284.5927 | 18.4917 | -0.0035 | 0.0908 | 0.0099 | -0.0015 | 0.0000 | -0.0110 | 46 | 1.4 | 1.0 |
| | 0.000094 | 0.0011 | 0.0030 | 0.0049 | 0.0051 | 0.0050 | 0.0039 | 0.0036 | 0.0040 | | | |

Table S1: Continued.

| ***Gaia*** **DR3** | $P$ | $T_0$ | $\overline{G}$ | $a_{1c}$ | $a_{2c}$ | $a_{3c}$ | $a_{1s}$ | $a_{2s}$ | $a_{3s}$ | $N$ | $\hat{q}_{\rm min}$ | $\hat{q}_{\rm min}^{-1\sigma}$ |
|---|---|---|---|---|---|---|---|---|---|---|---|---|
| | $P_{\rm err}$ | $T_{0,\rm err}$ | $\overline{G}_{\rm err}$ | $a_{1c,\rm err}$ | $a_{2c,\rm err}$ | $a_{3c,\rm err}$ | $a_{1s,\rm err}$ | $a_{2s,\rm err}$ | $a_{3s,\rm err}$ | | | |
| | [day] | BJD − 2455197.5 | [mag] | [mag] | [mag] | [mag] | [mag] | [mag] | [mag] | | | |
| 4515508300374125056 | 0.368973 | 2153.6964 | 18.2387 | -0.0092 | 0.0907 | -0.0011 | -0.0146 | 0.0000 | -0.0050 | 39 | 1.4 | 1.0 |
| | 0.000084 | 0.0013 | 0.0028 | 0.0042 | 0.0042 | 0.0043 | 0.0039 | 0.0039 | 0.0039 | | | |
| 4111214610668581376 | 0.50810 | 2308.7655 | 18.3752 | 0.0129 | 0.0907 | -0.0110 | -0.0126 | 0.0000 | 0.0046 | 43 | 1.4 | 1.0 |
| | 0.00019 | 0.0019 | 0.0031 | 0.0046 | 0.0049 | 0.0044 | 0.0047 | 0.0045 | 0.0049 | | | |
| 4281707976043168384 | 0.57959 | 2105.6485 | 18.0342 | -0.0180 | 0.0907 | -0.0077 | 0.0075 | 0.0000 | -0.0068 | 43 | 1.4 | 1.0 |
| | 0.00028 | 0.0019 | 0.0027 | 0.0034 | 0.0035 | 0.0034 | 0.0042 | 0.0038 | 0.0039 | | | |
| 4120093240073972864 | 0.52718 | 2378.9015 | 18.8404 | 0.0031 | 0.0907 | 0.0120 | -0.0063 | 0.0000 | -0.0004 | 45 | 1.4 | 1.0 |
| | 0.00017 | 0.0016 | 0.0026 | 0.0041 | 0.0037 | 0.0038 | 0.0031 | 0.0036 | 0.0034 | | | |
| 5833662969298401024 | 0.37362 | 2197.14520 | 17.6827 | 0.0067 | 0.0906 | -0.0039 | -0.0054 | 0.0000 | -0.0019 | 48 | 1.4 | 1.0 |
| | 0.00011 | 0.00091 | 0.0019 | 0.0030 | 0.0031 | 0.0025 | 0.0025 | 0.0025 | 0.0033 | | | |
| 5847314166394061184 | 0.258907 | 2194.04619 | 18.5408 | 0.0094 | 0.0906 | 0.0034 | -0.0265 | 0.0000 | 0.0029 | 47 | 1.4 | 1.0 |
| | 0.000050 | 0.00085 | 0.0027 | 0.0039 | 0.0036 | 0.0038 | 0.0035 | 0.0037 | 0.0034 | | | |
| 2056187834598367232 | 0.57763 | 2233.9778 | 17.8711 | -0.0036 | 0.0906 | 0.0025 | -0.0024 | 0.0000 | 0.0110 | 42 | 1.4 | 1.1 |
| | 0.00023 | 0.0011 | 0.0015 | 0.0021 | 0.0023 | 0.0018 | 0.0022 | 0.0021 | 0.0025 | | | |
| 4506469700652006656 | 0.74840 | 2185.7816 | 16.9831 | -0.0192 | 0.0905 | -0.0104 | -0.0021 | 0.0000 | -0.0037 | 29 | 1.4 | 1.0 |
| | 0.00055 | 0.0017 | 0.0020 | 0.0028 | 0.0027 | 0.0026 | 0.0025 | 0.0027 | 0.0026 | | | |
| 5836453323656146048 | 0.46730 | 2180.43051 | 17.7597 | -0.0126 | 0.0905 | -0.0019 | -0.0007 | 0.0000 | -0.0056 | 59 | 1.4 | 1.1 |
| | 0.00016 | 0.00099 | 0.0017 | 0.0028 | 0.0025 | 0.0027 | 0.0020 | 0.0023 | 0.0022 | | | |
| 5525928837412826624 | 0.40729 | 2210.7510 | 19.3407 | 0.0090 | 0.0905 | 0.0038 | 0.0148 | 0.0000 | 0.0007 | 45 | 1.4 | 1.0 |
| | 0.00012 | 0.0021 | 0.0039 | 0.0062 | 0.0049 | 0.0045 | 0.0049 | 0.0059 | 0.0056 | | | |
| 5884915539898670464 | 1.03953 | 2190.6752 | 18.0283 | 0.0229 | 0.0904 | 0.0167 | -0.0068 | 0.0000 | 0.0070 | 41 | 1.4 | 1.0 |
| | 0.00086 | 0.0037 | 0.0028 | 0.0039 | 0.0038 | 0.0040 | 0.0040 | 0.0042 | 0.0038 | | | |
| 4322097779775468800 | 0.355248 | 2181.27068 | 17.9007 | 0.0072 | 0.0904 | 0.0040 | 0.0045 | 0.0000 | 0.0012 | 39 | 1.4 | 1.0 |
| | 0.000082 | 0.00070 | 0.0017 | 0.0024 | 0.0026 | 0.0026 | 0.0024 | 0.0022 | 0.0023 | | | |
| 4111720081094185600 | 0.74586 | 2320.0609 | 18.2949 | -0.0120 | 0.0904 | -0.0066 | -0.0030 | 0.0000 | -0.0033 | 52 | 1.4 | 1.0 |
| | 0.00046 | 0.0015 | 0.0017 | 0.0021 | 0.0023 | 0.0020 | 0.0024 | 0.0023 | 0.0026 | | | |
| 5993175653779697408 | 0.343801 | 2262.74255 | 18.5579 | 0.0104 | 0.0904 | 0.0065 | -0.0196 | 0.0000 | 0.0026 | 55 | 1.4 | 1.0 |
| | 0.000071 | 0.00098 | 0.0023 | 0.0036 | 0.0040 | 0.0038 | 0.0032 | 0.0031 | 0.0034 | | | |
| 4340539514648010368 | 0.250363 | 2172.5099 | 18.3897 | -0.0065 | 0.0903 | -0.0033 | 0.0163 | 0.0000 | 0.0085 | 49 | 1.4 | 1.0 |
| | 0.000052 | 0.0014 | 0.0056 | 0.0053 | 0.0041 | 0.0049 | 0.0056 | 0.0062 | 0.0063 | | | |

Table S1: Continued.

| ***Gaia* DR3** | $P$ | $T_0$ | $\overline{G}$ | $a_{1c}$ | $a_{2c}$ | $a_{3c}$ | $a_{1s}$ | $a_{2s}$ | $a_{3s}$ | $N$ | $\hat{q}_{\rm min}$ | $\hat{q}_{\rm min}^{-1\sigma}$ |
|---|---|---|---|---|---|---|---|---|---|---|---|---|
| | $P_{\rm err}$ | $T_{0,\rm err}$ | $\overline{G}_{\rm err}$ | $a_{1c,\rm err}$ | $a_{2c,\rm err}$ | $a_{3c,\rm err}$ | $a_{1s,\rm err}$ | $a_{2s,\rm err}$ | $a_{3s,\rm err}$ | | | |
| | [day] | BJD − 2455197.5 | [mag] | [mag] | [mag] | [mag] | [mag] | [mag] | [mag] | | | |
| 5887458809069673344 | 0.59334 | 2144.9339 | 18.8501 | 0.0157 | 0.0903 | 0.0012 | -0.0010 | 0.0000 | -0.0006 | 41 | 1.4 | 1.0 |
| | 0.00028 | 0.0020 | 0.0027 | 0.0037 | 0.0037 | 0.0041 | 0.0037 | 0.0039 | 0.0038 | | | |
| 3403528932292557952 | 0.52689 | 2393.4995 | 18.3607 | 0.0165 | 0.0903 | -0.0053 | -0.0077 | 0.0000 | 0.0068 | 43 | 1.4 | 1.0 |
| | 0.00018 | 0.0017 | 0.0026 | 0.0037 | 0.0040 | 0.0030 | 0.0037 | 0.0032 | 0.0042 | | | |
| 5980205947768977280 | 0.68675 | 2331.0451 | 17.4642 | -0.0035 | 0.0902 | 0.0059 | -0.0005 | 0.0000 | 0.0037 | 34 | 1.4 | 1.0 |
| | 0.00038 | 0.0011 | 0.0014 | 0.0020 | 0.0022 | 0.0019 | 0.0021 | 0.0018 | 0.0021 | | | |
| 6019891479940114944 | 0.58280 | 2321.5005 | 18.4539 | 0.0080 | 0.0902 | 0.0102 | 0.0034 | 0.0000 | -0.0026 | 49 | 1.4 | 1.0 |
| | 0.00028 | 0.0017 | 0.0023 | 0.0034 | 0.0035 | 0.0029 | 0.0032 | 0.0031 | 0.0037 | | | |
| 251739234495031936 | 0.51267 | 2111.6414 | 18.0559 | -0.0092 | 0.0902 | 0.0033 | -0.0047 | 0.0000 | 0.0031 | 46 | 1.4 | 1.0 |
| | 0.00021 | 0.0012 | 0.0017 | 0.0025 | 0.0021 | 0.0026 | 0.0022 | 0.0026 | 0.0021 | | | |
| 4117363908727669760 | 0.79902 | 2404.7088 | 18.6146 | -0.0190 | 0.0902 | 0.0016 | 0.0068 | 0.0000 | 0.0065 | 43 | 1.4 | 1.0 |
| | 0.00033 | 0.0029 | 0.0031 | 0.0043 | 0.0043 | 0.0041 | 0.0041 | 0.0039 | 0.0038 | | | |
| 5930627907700568320 | 0.322787 | 2193.15833 | 17.6523 | 0.0044 | 0.0902 | 0.0049 | -0.0094 | 0.0000 | 0.0006 | 52 | 1.4 | 1.0 |
| | 0.000068 | 0.00083 | 0.0018 | 0.0027 | 0.0033 | 0.0030 | 0.0029 | 0.0025 | 0.0028 | | | |
| 4118863500745320064 | 1.11020 | 2400.7877 | 17.6203 | -0.0231 | 0.0902 | -0.0049 | 0.0012 | 0.0000 | 0.0062 | 42 | 1.4 | 1.0 |
| | 0.00089 | 0.0028 | 0.0018 | 0.0028 | 0.0027 | 0.0025 | 0.0025 | 0.0026 | 0.0027 | | | |
| 5983948071186821376 | 0.96239 | 2094.2196 | 17.6300 | 0.0119 | 0.0901 | -0.0036 | 0.0050 | 0.0000 | 0.0005 | 60 | 1.4 | 1.0 |
| | 0.00063 | 0.0020 | 0.0018 | 0.0027 | 0.0031 | 0.0028 | 0.0027 | 0.0023 | 0.0027 | | | |
| 2034671732104144000 | 0.283357 | 2210.58085 | 17.9951 | 0.0197 | 0.0901 | 0.0029 | 0.0042 | 0.0000 | -0.0008 | 50 | 1.4 | 1.0 |
| | 0.000057 | 0.00056 | 0.0018 | 0.0027 | 0.0029 | 0.0026 | 0.0021 | 0.0022 | 0.0025 | | | |
| 5891711758737858176 | 1.00313 | 2185.1453 | 17.9852 | 0.0087 | 0.0901 | 0.0150 | -0.0002 | 0.0000 | -0.0025 | 59 | 1.4 | 1.0 |
| | 0.00045 | 0.0028 | 0.0024 | 0.0032 | 0.0039 | 0.0033 | 0.0038 | 0.0029 | 0.0037 | | | |
| 4067808571662706688 | 0.60752 | 2410.2267 | 16.9705 | -0.0050 | 0.0901 | 0.0015 | 0.0109 | 0.0000 | 0.0004 | 39 | 1.4 | 1.0 |
| | 0.00026 | 0.0013 | 0.0021 | 0.0025 | 0.0032 | 0.0026 | 0.0034 | 0.0025 | 0.0032 | | | |
| 5932862664994144128 | 0.55352 | 2197.1331 | 18.3145 | 0.0129 | 0.0900 | -0.0034 | 0.0053 | 0.0000 | -0.0016 | 58 | 1.4 | 1.0 |
| | 0.00025 | 0.0014 | 0.0021 | 0.0029 | 0.0030 | 0.0029 | 0.0030 | 0.0029 | 0.0030 | | | |
| 5875909886869867008 | 0.75001 | 2225.8778 | 18.2061 | 0.0152 | 0.0898 | -0.0008 | -0.0069 | 0.0000 | -0.0050 | 43 | 1.4 | 1.0 |
| | 0.00042 | 0.0026 | 0.0031 | 0.0037 | 0.0035 | 0.0042 | 0.0036 | 0.0039 | 0.0037 | | | |
| 4057416129538784640 | 0.397563 | 2377.0960 | 18.2611 | 0.0153 | 0.0898 | -0.0063 | 0.0047 | 0.0000 | -0.0027 | 40 | 1.4 | 1.0 |
| | 0.000092 | 0.0012 | 0.0025 | 0.0039 | 0.0034 | 0.0041 | 0.0033 | 0.0034 | 0.0028 | | | |

Table S1: Continued.

| ***Gaia*** DR3 | $P$<br>$P_{\rm err}$<br>[day] | $T_0$<br>$T_{0,\rm err}$<br>BJD − 2455197.5 | $\overline{G}$<br>$\overline{G}_{\rm err}$<br>[mag] | $a_{1\rm c}$<br>$a_{1\rm c,err}$<br>[mag] | $a_{2\rm c}$<br>$a_{2\rm c,err}$<br>[mag] | $a_{3\rm c}$<br>$a_{3\rm c,err}$<br>[mag] | $a_{1\rm s}$<br>$a_{1\rm s,err}$<br>[mag] | $a_{2\rm s}$<br>$a_{2\rm s,err}$<br>[mag] | $a_{3\rm s}$<br>$a_{3\rm s,err}$<br>[mag] | $N$ | $\hat{q}_{\rm min}$ | $\hat{q}_{\rm min}^{-1\sigma}$ |
|---|---|---|---|---|---|---|---|---|---|---|---|---|
| 5870863094153430144 | 0.82485 | 2194.6947 | 17.0445 | -0.0248 | 0.0898 | -0.0057 | 0.0054 | 0.0000 | -0.0015 | 47 | 1.4 | 1.0 |
| | 0.00047 | 0.0019 | 0.0019 | 0.0028 | 0.0028 | 0.0024 | 0.0026 | 0.0025 | 0.0031 | | | |
| 5951023328613748224 | 0.65922 | 2239.6565 | 17.5573 | 0.0143 | 0.0897 | 0.0023 | 0.0011 | 0.0000 | -0.0021 | 37 | 1.4 | 1.0 |
| | 0.00038 | 0.0017 | 0.0021 | 0.0032 | 0.0031 | 0.0030 | 0.0027 | 0.0028 | 0.0028 | | | |
| 1827494570016143232 | 0.64416 | 2169.3121 | 18.4896 | -0.0052 | 0.0897 | 0.0020 | -0.0107 | 0.0000 | -0.0019 | 39 | 1.4 | 1.0 |
| | 0.00033 | 0.0015 | 0.0019 | 0.0027 | 0.0026 | 0.0026 | 0.0027 | 0.0028 | 0.0026 | | | |
| 4117020345704069760 | 1.11632 | 2416.6376 | 18.3325 | -0.0139 | 0.0896 | -0.0101 | 0.0022 | 0.0000 | 0.0006 | 41 | 1.4 | 1.0 |
| | 0.00077 | 0.0032 | 0.0022 | 0.0031 | 0.0032 | 0.0032 | 0.0031 | 0.0033 | 0.0034 | | | |
| 4303135774045677952 | 0.68752 | 2112.4090 | 17.8086 | -0.0059 | 0.0895 | -0.0040 | -0.0023 | 0.0000 | -0.0099 | 41 | 1.4 | 1.0 |
| | 0.00033 | 0.0018 | 0.0021 | 0.0027 | 0.0027 | 0.0025 | 0.0031 | 0.0029 | 0.0028 | | | |
| 5516255540272479744 | 0.67690 | 2217.3634 | 17.8357 | 0.0079 | 0.0894 | -0.0002 | 0.0038 | 0.0000 | 0.0017 | 41 | 1.4 | 1.0 |
| | 0.00032 | 0.0015 | 0.0019 | 0.0028 | 0.0028 | 0.0026 | 0.0025 | 0.0024 | 0.0025 | | | |
| 4121520023917835904 | 0.62882 | 2459.3046 | 17.9100 | 0.0121 | 0.0893 | 0.0068 | 0.0002 | 0.0000 | -0.0002 | 53 | 1.4 | 1.0 |
| | 0.00023 | 0.0014 | 0.0018 | 0.0025 | 0.0025 | 0.0025 | 0.0024 | 0.0025 | 0.0026 | | | |

Table S1: Continued.
